# Supplementary material for: SVFSearch: A Multimodal Knowledge-Intensive Benchmark for Short-Video Frame Search in the Gaming Vertical Domain
Source: arXiv:2605.17946 source file (2026-05-20)
Supplement: Supplementary file 1 [file A.related_works.tex]

\section{Related Work}
\label{sec:related_work}

\paragraph{Multimodal Benchmarks: from VQA to Multimodal Search.}
Visual question answering has evolved from open-ended image QA
\citep{antol2015vqa,goyal2017making}
to more specialized settings such as scene-text understanding,
science reasoning, and knowledge-intensive QA
\citep{singh2019towards,lu2022learn,marino2019ok}.
In parallel, broad multimodal benchmarks including
MMBench, MME, MM-Vet, and MMMU-Pro
\citep{liu2024mmbench,fu2023mme,yu2023mm,yue2024mmmu,yue2025mmmu}
have become common testbeds for evaluating frontier MLLMs.
More recently, several benchmarks have moved toward
\emph{multimodal retrieval and search}, covering multi-hop web QA
\citep{chang2022webqa}, vision-centric mRAG \citep{hu2024mrag},
adaptive retrieval planning \citep{li2024benchmarking},
and multimodal search engines
\citep{jiang2024mmsearch,tao2025mmsearch,yu2025mramg}.
Despite this progress, existing multimodal search benchmarks mainly focus on
general-domain image-question inputs or web-search settings. These settings do
not fully match short-video frame search, where a user question is grounded in
a paused video frame and may be accompanied by noisy video-side context, such
as the cover image, title, OCR text, and ASR transcript. The relevant evidence
may also be scattered across domain-specific and rapidly changing sources. This
gap is especially pronounced in the gaming vertical, where characters, items,
mechanics, events, and patches evolve quickly and are rarely covered by stable,
structured knowledge bases. \bench~targets this setting by evaluating
game-scene understanding and retrieval-augmented QA over paused-frame images,
with frozen text, image, and multimodal retrieval resources.

\paragraph{Agentic Multimodal Search.}
Agentic search methods provide a natural evaluation setting for multimodal
search benchmarks, since models must decide when and how to use external tools
before answering. One line of work follows the ReAct-style paradigm
\citep{yao2022react}, decomposing a query into planning, tool invocation,
evidence aggregation, and answer generation. This paradigm is well matched to
\bench, where questions may require visual grounding, text retrieval,
multimodal retrieval, and domain knowledge lookup. We therefore implement a
LangGraph-based Plan-Act-Replan baseline with domain-specific retrieval tools. A second line trains search agents with outcome-based RL. Built on R1-style
reasoning and GRPO \citep{guo2025deepseek,shao2024deepseekmath}, Search-R1 and
its variants \citep{jin2025search,song2025r1,chen2503research} study text-based
search agents, while MMSearch-R1 \citep{wu2025mmsearch} extends this paradigm to
on-demand multimodal web search. DeepMMSearch-R1
\citep{narayan2025deepmmsearch} further relaxes single-call and whole-image
constraints. We adapt this line to the game-domain multiple-choice setting by
training an MMSearch-R1-style model and using it as a learned search baseline.
Together, these baselines provide complementary references for evaluating
retrieval-augmented and agentic multimodal search on \bench.
