# Supplementary material for: SVFSearch: A Multimodal Knowledge-Intensive Benchmark for Short-Video Frame Search in the Gaming Vertical Domain
Source: arXiv:2605.17946 source file (2026-05-20)
Supplement: Supplementary file 2 [file B.extend_benchmark_analyse.tex]

\section{Additional Experimental Results}
\label{app:additional_results}

\begin{table*}[!htbp]
\centering
\scriptsize
\setlength{\tabcolsep}{2.4pt}
\caption{%
  \textbf{Comprehensive results on \bench.}
  Results are reported on the 5,000-example test split.
  \textbf{SR} denotes the fraction of examples where the system invokes at
  least one retrieval tool; ``---'' indicates settings without \bench{}
  retrieval tools.
  $^{\dagger}$ denotes native thinking mode.
  \best{Bold} marks the best overall accuracy within each setting block.}
\label{tab:full_results}
\resizebox{\textwidth}{!}{%
\begin{tabular}{llccccccccccc}
\toprule
& & \multicolumn{1}{c}{\textbf{Overall}}
& \multicolumn{1}{c}{\textbf{Search}}
& \multicolumn{6}{c}{\textbf{Category}}
& \multicolumn{3}{c}{\textbf{Difficulty}} \\
\cmidrule(lr){3-3}\cmidrule(lr){4-4}\cmidrule(lr){5-10}\cmidrule(lr){11-13}
\textbf{Setting} & \textbf{Model}
& \textbf{Acc.} & \textbf{SR}
& \textbf{Char.} & \textbf{Equip.} & \textbf{Map} & \textbf{Story} & \textbf{Mech.} & \textbf{Other}
& \textbf{Easy} & \textbf{Med.} & \textbf{Hard} \\
\midrule

\multicolumn{13}{l}{\cellcolor{lightgray}\textit{Proprietary Models (Direct QA)}} \\
Direct & Claude-Opus-4.7 & 69.0 & --- & 70.0 & 69.0 & 66.8 & 72.7 & 66.2 & 66.7 & 67.9 & 68.6 & 72.9 \\
Direct & GPT-5.4 & 67.9 & --- & 69.8 & 67.8 & 59.7 & 69.7 & 63.7 & 66.7 & 65.1 & 67.7 & 70.4 \\
Direct & \best{Gemini-3.1-Pro} & \best{77.5} & --- & 79.1 & 79.6 & 69.9 & 87.9 & 72.3 & 71.4 & 82.5 & 78.3 & 68.2 \\
\midrule

\multicolumn{13}{l}{\cellcolor{lightgray}\textit{Open-source Direct QA}} \\
Direct & Qwen2.5-VL-7B & 49.8 & --- & 50.8 & 47.9 & 47.4 & 51.5 & 48.1 & 57.1 & 57.1 & 49.4 & 50.2 \\
Direct & Qwen2.5-VL-7B-CoT & 47.4 & --- & 47.8 & 47.6 & 46.4 & 60.6 & 45.8 & 42.9 & 64.6 & 47.5 & 39.3 \\
Direct & Qwen3-VL-2B & 33.1 & --- & 34.2 & 32.5 & 27.6 & 27.3 & 31.3 & 38.1 & 34.9 & 31.6 & 44.9 \\
Direct & Qwen3-VL-2B-Thinking & 47.8 & --- & 49.2 & 45.1 & 49.5 & 48.5 & 45.7 & 33.3 & 62.3 & 46.9 & 49.8 \\
Direct & Qwen3-VL-4B & 52.9 & --- & 53.7 & 52.3 & 50.0 & 69.7 & 51.2 & 57.1 & 67.9 & 52.2 & 53.2 \\
Direct & Qwen3-VL-4B-Thinking & 54.2 & --- & 54.5 & 51.9 & 58.7 & 51.5 & 54.8 & 38.1 & 71.7 & 53.4 & 53.8 \\
Direct & Qwen3-VL-8B & 54.8 & --- & 56.5 & 52.4 & 55.1 & 66.7 & 50.9 & 47.6 & 58.0 & 53.8 & 61.9 \\
Direct & Qwen3-VL-8B-Thinking & 53.7 & --- & 54.1 & 54.0 & 52.0 & 60.6 & 52.0 & 61.9 & 74.1 & 52.8 & 52.8 \\
Direct & Qwen3-VL-32B & 57.1 & --- & 58.7 & 54.3 & 53.6 & 63.6 & 54.4 & 71.4 & 71.2 & 56.2 & 58.9 \\
Direct & Qwen3-VL-32B-Thinking & 62.2 & --- & 63.4 & 60.9 & 58.2 & 69.7 & 59.8 & 76.2 & 75.5 & 61.9 & 59.9 \\
Direct & Qwen3.5-0.8B & 34.1 & --- & 34.4 & 32.2 & 32.1 & 30.3 & 34.8 & 42.9 & 45.3 & 33.7 & 32.4 \\
Direct & Qwen3.5-0.8B$^{\dagger}$ & 42.8 & --- & 45.4 & 37.2 & 41.8 & 27.3 & 39.4 & 47.6 & 52.4 & 41.5 & 49.8 \\
Direct & Qwen3.5-2B & 56.5 & --- & 55.6 & 57.9 & 58.7 & 51.5 & 57.7 & 71.4 & 63.2 & 56.1 & 56.7 \\
Direct & Qwen3.5-2B$^{\dagger}$ & 49.3 & --- & 50.2 & 45.7 & 51.0 & 30.3 & 49.1 & 61.9 & 63.2 & 47.9 & 54.9 \\
Direct & Qwen3.5-4B & 57.3 & --- & 57.8 & 57.8 & 53.1 & 66.7 & 56.0 & 61.9 & 69.8 & 55.9 & 63.6 \\
Direct & Qwen3.5-4B$^{\dagger}$ & 59.1 & --- & 60.7 & 55.1 & 54.6 & 51.5 & 58.6 & 42.8 & 66.5 & 58.2 & 63.6 \\
Direct & Qwen3.5-9B & 59.9 & --- & 61.1 & 57.1 & 57.1 & 60.6 & 58.6 & 66.7 & 59.9 & 59.2 & 65.4 \\
Direct & Qwen3.5-9B$^{\dagger}$ & 58.3 & --- & 59.3 & 55.7 & 61.2 & 66.7 & 56.6 & 57.1 & 63.7 & 57.6 & 62.3 \\
Direct & \best{Qwen3.5-27B} & \best{66.4} & --- & 68.0 & 63.1 & 63.8 & 75.8 & 63.9 & 76.2 & 73.6 & 65.5 & 71.3 \\
Direct & Qwen3.5-27B$^{\dagger}$ & 64.8 & --- & 65.4 & 62.5 & 61.2 & 72.7 & 64.8 & 66.7 & 69.8 & 64.8 & 62.5 \\
\midrule

\multicolumn{13}{l}{\cellcolor{lightgray}\textit{Open-source RAG Workflow}} \\
Workflow & Qwen2.5-VL-7B & 57.3 & 100.0 & 57.7 & 58.6 & 58.2 & 69.7 & 54.3 & 52.4 & 59.4 & 57.9 & 51.0 \\
Workflow & Qwen3-VL-2B & 47.1 & 100.0 & 47.1 & 48.3 & 49.5 & 45.5 & 46.1 & 28.6 & 48.6 & 47.2 & 45.1 \\
Workflow & Qwen3-VL-4B & 57.6 & 100.0 & 57.2 & 60.4 & 58.2 & 60.6 & 56.5 & 61.9 & 70.8 & 58.2 & 47.2 \\
Workflow & Qwen3-VL-8B & 63.5 & 100.0 & 64.1 & 66.5 & 63.3 & 60.6 & 59.6 & 61.9 & 66.5 & 64.3 & 55.3 \\
Workflow & Qwen3-VL-32B & 62.2 & 100.0 & 61.6 & 67.2 & 62.8 & 69.7 & 60.3 & 61.9 & 78.3 & 62.7 & 51.4 \\
Workflow & Qwen3.5-0.8B & 33.0 & 100.0 & 33.9 & 30.3 & 35.7 & 30.3 & 31.6 & 33.3 & 40.1 & 33.0 & 29.4 \\
Workflow & Qwen3.5-2B & 44.0 & 100.0 & 44.3 & 46.6 & 38.3 & 45.5 & 42.5 & 23.8 & 56.1 & 44.8 & 32.4 \\
Workflow & Qwen3.5-4B & 56.5 & 100.0 & 57.9 & 53.5 & 53.6 & 63.6 & 55.0 & 47.6 & 61.8 & 56.8 & 52.2 \\
Workflow & Qwen3.5-9B & 66.5 & 100.0 & 67.5 & 67.2 & 64.3 & 63.6 & 63.3 & 61.9 & 70.8 & 66.5 & 64.4 \\
Workflow & \best{Qwen3.5-27B} & \best{69.4} & 100.0 & 70.8 & 69.4 & 65.8 & 78.8 & 65.3 & 66.7 & 70.8 & 69.1 & 71.0 \\
\midrule

\multicolumn{13}{l}{\cellcolor{lightgray}\textit{Open-source Plan-Act-Replan Agent}} \\
PAR & Qwen2.5-VL-7B & 59.3 & 85.6 & 59.3 & 61.7 & 63.3 & 54.5 & 56.9 & 52.4 & 55.2 & 59.8 & 56.5 \\
PAR & Qwen3-VL-2B & 50.9 & 100.0 & 50.3 & 53.2 & 53.1 & 54.5 & 50.6 & 42.9 & 52.4 & 51.4 & 45.9 \\
PAR & Qwen3-VL-8B & 63.7 & 99.7 & 62.8 & 66.1 & 70.9 & 63.6 & 63.2 & 66.7 & 66.5 & 64.2 & 58.3 \\
PAR & Qwen3-VL-32B & 71.6 & 98.4 & 71.1 & 75.9 & 74.5 & 69.7 & 69.4 & 76.2 & 79.7 & 72.4 & 61.5 \\
PAR & Qwen3.5-2B & 44.7 & 99.3 & 44.8 & 48.1 & 40.8 & 48.5 & 42.6 & 28.6 & 55.7 & 45.5 & 33.4 \\
PAR & Qwen3.5-4B & 67.7 & 98.1 & 67.5 & 69.7 & 68.4 & 69.7 & 66.4 & 71.4 & 65.6 & 68.1 & 65.4 \\
PAR & \best{Qwen3.5-9B} & \best{79.1} & 100.0 & 79.3 & 82.7 & 79.1 & 87.9 & 76.0 & 71.4 & 75.0 & 79.7 & 75.9 \\
PAR & Qwen3.5-27B & 78.6 & 96.8 & 78.3 & 83.1 & 81.1 & 81.8 & 75.5 & 81.0 & 79.7 & 79.0 & 74.5 \\
\midrule

\multicolumn{13}{l}{\cellcolor{lightgray}\textit{Open-source MMSearch-R1 Search Models}} \\
MS-R1 & Qwen2.5-VL-7B & 49.4 & 72.8 & 49.1 & 53.8 & 54.1 & 60.6 & 46.2 & 33.3 & 49.1 & 35.5 & 29.8 \\
MS-R1 & Qwen3-VL-8B & 63.2 & 0.02 & 64.5 & 60.8 & 63.3 & 63.6 & 61.1 & 52.4 & 70.3 & 62.6 & 65.6 \\
MS-R1-Game & \best{Qwen3-VL-8B} & \best{64.5} & 68.2 & 65.2 & 66.8 & 65.3 & 63.6 & 60.0 & 76.2 & 73.6 & 64.3 & 61.9 \\
\midrule

\multicolumn{13}{l}{\cellcolor{lightgray}\textit{Open-source Oracle Knowledge (Upper Bound)}} \\
Oracle & Qwen2.5-VL-7B & 76.0 & --- & 78.0 & 78.5 & 81.6 & 84.9 & 67.6 & 47.6 & 63.7 & 77.4 & 69.4 \\
Oracle & Qwen3-VL-2B & 52.3 & --- & 50.3 & 61.9 & 61.7 & 57.6 & 49.8 & 38.1 & 44.3 & 52.3 & 55.9 \\
Oracle & Qwen3-VL-4B & 84.6 & --- & 86.7 & 87.7 & 82.7 & 90.9 & 76.6 & 57.1 & 77.4 & 85.3 & 81.6 \\
Oracle & Qwen3-VL-8B & 86.5 & --- & 88.4 & 87.5 & 87.8 & 78.8 & 80.3 & 76.2 & 73.1 & 87.5 & 84.0 \\
Oracle & Qwen3-VL-32B & 90.8 & --- & 92.0 & 94.1 & 88.3 & 93.9 & 85.4 & 81.0 & 87.7 & 91.4 & 87.0 \\
Oracle & Qwen3.5-0.8B & 25.8 & --- & 25.4 & 30.2 & 22.5 & 18.2 & 24.7 & 33.3 & 32.1 & 26.4 & 18.2 \\
Oracle & Qwen3.5-2B & 68.5 & --- & 67.5 & 75.3 & 66.8 & 66.7 & 66.6 & 81.0 & 76.9 & 69.2 & 59.5 \\
Oracle & Qwen3.5-4B & 87.9 & --- & 88.4 & 90.7 & 86.7 & 81.8 & 84.9 & 76.2 & 86.3 & 88.4 & 84.4 \\
Oracle & Qwen3.5-9B & 90.3 & --- & 90.7 & 91.9 & 86.2 & 97.0 & 88.4 & 85.7 & 91.5 & 90.7 & 85.8 \\
Oracle & \best{Qwen3.5-27B} & \best{95.4} & --- & 96.0 & 96.7 & 95.9 & 87.9 & 93.0 & 90.5 & 94.3 & 95.7 & 93.5 \\
\bottomrule
\end{tabular}%
}
\end{table*}

\subsection{Full Results on \bench}
\label{app:full_results}

Table~\ref{tab:full_results} extends Table~\ref{tab:main_results} with
additional model scales. The same trends remain: Direct QA is limited,
retrieval-augmented settings improve performance when the backbone can use
external evidence, and Oracle Knowledge provides a much higher upper bound.
The results also show that \bench{} is challenging across model families.
Larger and newer models generally perform better, but sizable Oracle gaps
remain, indicating persistent failures in visual grounding, retrieval quality, evidence integration, and evidence-grounded reasoning.

The extended results also reveal robustness issues that are less visible in the main table. Very small models are unstable in tool-augmented settings, consistent with the diagnostics in Section~\ref{sec:tool_use_diagnostics}: agentic search requires sufficient visual understanding, instruction following, and evidence integration. Native thinking mode is not uniformly helpful either. It improves some larger models but can degrade smaller ones, likely due to formatting errors or context drift. These observations complement the main analysis by showing how model scale and reasoning mode affect robustness on \bench{}.

\vspace{-1em}
\begin{figure}[t]
  \centering
  \includegraphics[width=\textwidth]{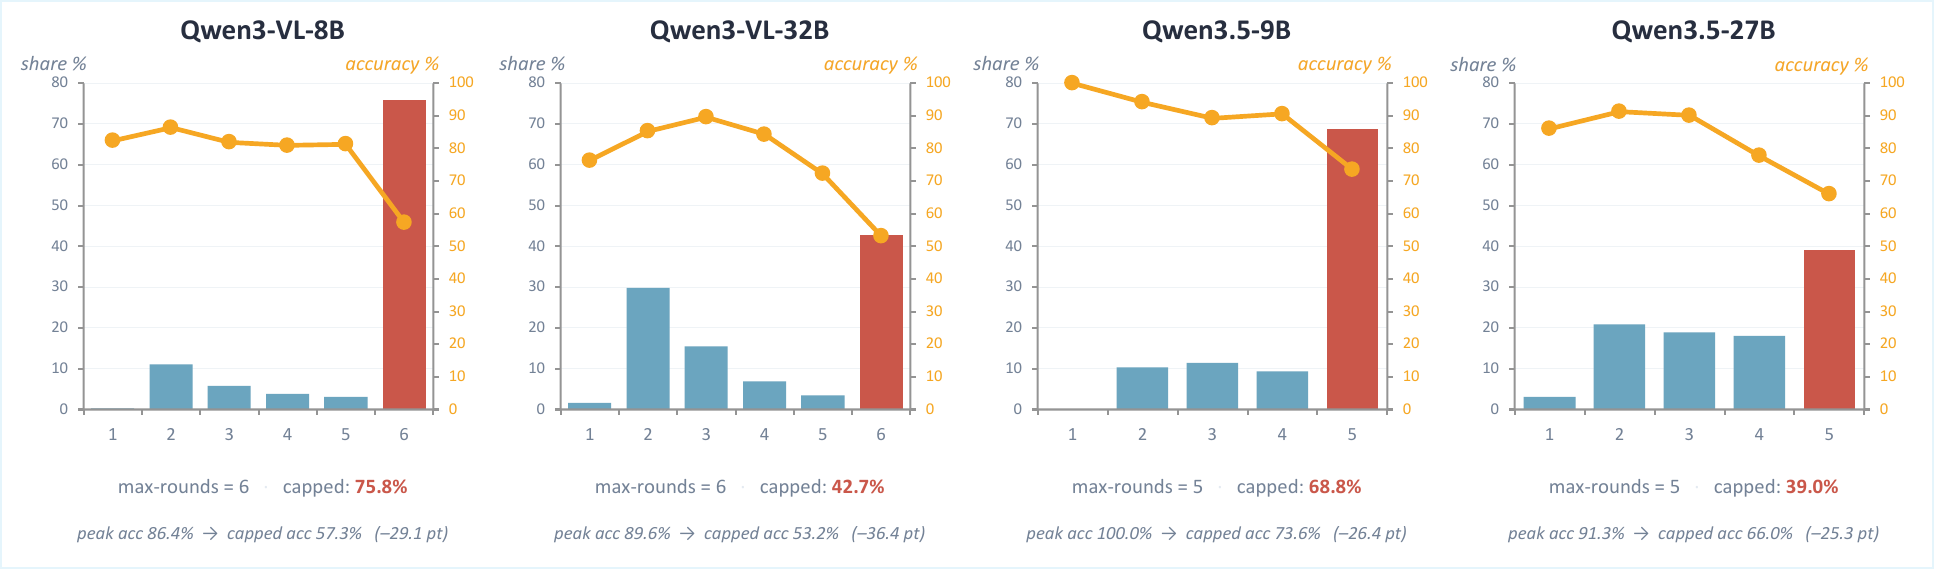}
    \caption{\textbf{Planning-round analysis under PAR.}
    Bars show the share of examples ending at each planning round, and lines show the corresponding accuracy. Red bars indicate examples capped by the maximum number of planning rounds.}
  \label{fig:plan_round_analysis}
  \vspace{-0.5em}
\end{figure}

\subsection{Planning-round Analysis}
\label{app:plan_round_analysis}

Figure~\ref{fig:plan_round_analysis} groups PAR examples by the planning round at which the agent stops. Accuracy usually improves after a few rounds but drops on late or capped cases. This suggests that moderate search can help evidence acquisition, while excessive planning often reflects unresolved uncertainty rather than better evidence use. Capped examples are typically harder cases where the agent fails in visual grounding, query formulation, or retrieval. These results suggest that PAR benefits from a limited number of search rounds, but simply extending the search process does not guarantee better answers.

\subsection{Retrieval Backend Analysis}
\label{app:retrieval_backend}

\begin{figure*}[t]
  \centering
  \includegraphics[width=\textwidth]{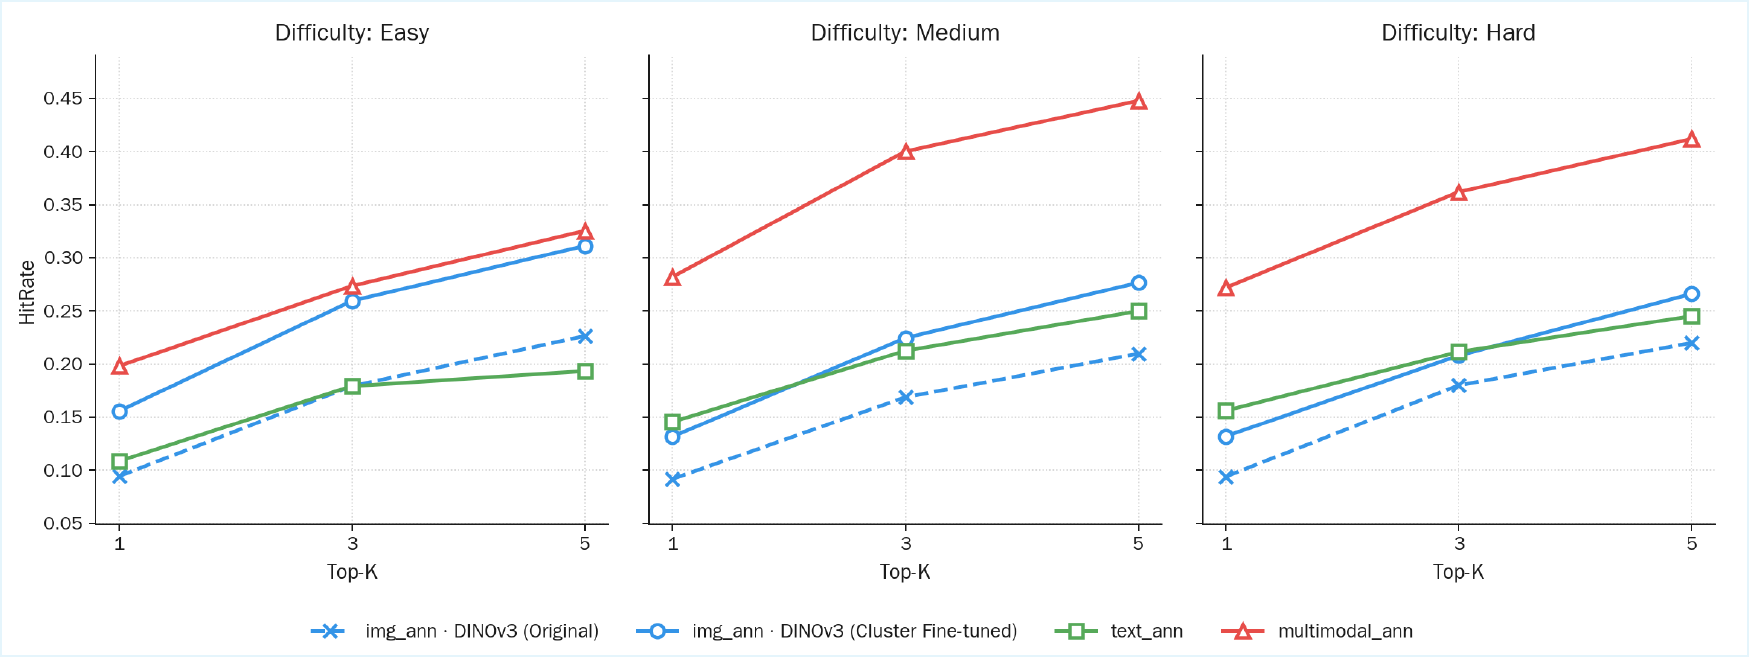}
    \caption{\textbf{HitRate@K of retrieval backends across difficulty levels.}
    We compare original DINOv3 image retrieval, cluster-aware fine-tuned DINOv3 image retrieval, text retrieval, and multimodal retrieval for $K \in \{1,3,5\}$.}
    \label{fig:retrieval_hitrate}
     \vspace{-1.5em}
\end{figure*}

Figure~\ref{fig:retrieval_hitrate} evaluates the frozen retrieval backends used by \bench. The cluster-aware DINOv3 fine-tuning described in Section~\ref{sec:image_retrieval_training} consistently improves image retrieval over the original DINOv3 encoder across difficulty levels and top-$K$ values. This shows that core-element-aware training helps align paused game frames with their target elements. The gain is moderate, since the same core element may appear with large visual variation in viewpoint, skin, UI state, background, and combat context, while different elements from the same game can also look similar.

Multimodal retrieval achieves the highest HitRate@K in most settings, especially on medium and hard examples. This indicates that combining visual and textual signals is more effective than relying on a single retrieval modality. The comparison should also be interpreted with model capacity in mind: the multimodal index uses Qwen3-VL-Embedding-2B, while the text index uses Qwen3-Embedding-0.6B and the image index uses the fine-tuned DINOv3-Base encoder. Overall, the results show that image, text, and multimodal retrieval provide complementary signals for \bench.
