# Supplementary material for: SVFSearch: A Multimodal Knowledge-Intensive Benchmark for Short-Video Frame Search in the Gaming Vertical Domain
Source: arXiv:2605.17946 source file (2026-05-20)
Supplement: Supplementary file 3 [file C.Algorithm_Flowchart.tex]

\definecolor{gaTeal}{HTML}{4E8E8A}
\definecolor{gaLightTeal}{HTML}{EDF6F5}
\definecolor{gaFrame}{HTML}{D8E2E7}
\definecolor{gaOrange}{HTML}{D97706}
\definecolor{gaLightOrange}{HTML}{FFF7ED}
\definecolor{gaBlue}{HTML}{4A78A8}
\definecolor{gaLightBlue}{HTML}{EEF5FB}

\newcommand{\field}[1]{\ifmmode\mathtt{#1}\else\texttt{#1}\fi}
\newcommand{\tool}[1]{\ifmmode\mathtt{#1}\else\texttt{#1}\fi}
\newcommand{\tagtok}[1]{\texttt{#1}}

\DefineVerbatimEnvironment{PromptVerb}{Verbatim}{
  fontsize=\scriptsize,
  breaklines=true,
  breakanywhere=true,
  tabsize=2
}

\newtcolorbox{systemcard}[2][]{
  enhanced jigsaw,
  breakable,
  colback=#2,
  colframe=gaFrame,
  boxrule=0.45pt,
  leftrule=2.2pt,
  arc=2pt,
  left=6pt,
  right=6pt,
  top=5pt,
  bottom=5pt,
  before skip=6pt,
  after skip=8pt,
  pad at break*=1.5mm,
  #1
}

\newcommand{\cardtitle}[2]{%
  \noindent{\small\bfseries\textcolor{#1}{#2}}\par\vspace{3pt}
}

% =============================================================================

\section{Implementation Details of Tool-Augmented Search Settings}
\label{app:tool_augmented_systems}

We provide implementation details for the three tool-augmented settings used in our evaluation: the fixed RAG workflow, the LangGraph-based PAR agent, and MS-R1-style search models. These settings share the same frozen offline retrieval environment, but differ in how retrieval actions are selected, tool observations are accumulated, and final answers are produced.

Because \bench~targets the Chinese gaming vertical, the actual implementation uses Chinese prompts and tool cards. The surrounding explanations are written in English, while the original Chinese prompts and skill cards are preserved verbatim in shaded implementation boxes. Machine-readable tags, tool names, endpoints, and JSON fields are kept unchanged throughout.

\subsection{Shared Offline Retrieval Tools}
\label{app:shared_retrieval_interfaces}

All tool-augmented settings access the same frozen retrieval resources. The retrieval tools operate offline and do not access live web search. This design makes the evaluation deterministic and allows us to compare search behavior under identical retrieval conditions.

% =============================================================================
\subsection{Fixed Retrieval-Augmented Generation Workflow}
\label{app:rag_workflow}

\paragraph{System description.}
The fixed RAG workflow follows a deterministic image-to-text retrieval chain. It first performs image retrieval to infer the most likely core element in the paused-frame image. The selected element is then concatenated with the original question to form a text retrieval query. Finally, the retrieved evidence is inserted into a multimodal answer prompt together with the image, question, and answer options.

\begin{algorithm}[H]
\caption{Fixed RAG Workflow}
\label{alg:appendix_rag}
\begin{algorithmic}[1]
\Require question $q$, options $O$, image $I$, retrieval depth $k$
\Ensure predicted answer $a^*$

\State \textbf{Image retrieval.}
\State $\mathcal{R}_{\mathrm{img}} \leftarrow \mathrm{ImgANN}(I,k)$

\State \textbf{Core-element selection.}
\State $C \leftarrow \{r.\mathrm{query} \mid r \in \mathcal{R}_{\mathrm{img}},\ r.\mathrm{query}\neq\emptyset\}$
\If{$C \neq \emptyset$}
    \State $Q^* \leftarrow \arg\max_{q' \in C}\ \mathrm{count}(q',C)$
    \Comment{majority vote over retrieved queries}
\Else
    \State $r^* \leftarrow \arg\max_{r \in \mathcal{R}_{\mathrm{img}}} r.\mathrm{score}$
    \State $Q^* \leftarrow r^*.\mathrm{query}$
    \Comment{fallback to the highest-scoring record}
\EndIf

\State \textbf{Text retrieval.}
\If{$Q^* \neq \emptyset$}
    \State $\mathcal{R}_{\mathrm{txt}} \leftarrow \mathrm{TextANN}(Q^* \oplus q,k)$
\Else
    \State $\mathcal{R}_{\mathrm{txt}} \leftarrow \mathrm{TextANN}(q,k)$
\EndIf
\Comment{$\oplus$ denotes string concatenation}

\State \textbf{Answer generation.}
\State $\mathcal{E} \leftarrow
\mathrm{ExtractTopK}(\mathcal{R}_{\mathrm{img}})
\cup
\mathrm{ExtractTopK}(\mathcal{R}_{\mathrm{txt}})$
\State $a^* \leftarrow \mathrm{MLLM}_{\mathrm{answer}}(I,q,O,\mathcal{E})$
\State \Return $a^*$
\end{algorithmic}
\end{algorithm}

\vspace{-1.5em}
\paragraph{Prompt template.}
The RAG answer prompt is intentionally concise. It presents the question,
candidate options, and retrieved knowledge, and asks the model to output only the full text of the selected option.

\begin{systemcard}{gaLightTeal}
\cardtitle{gaTeal}{RAG answer prompt: original implementation}
\begin{PromptVerb}
你是一个多模态游戏问答助手。根据图片和参考知识（如有）回答问题，并从给定选项中选择最正确的一项。

问题：
{question}

选项：
A. {option_1} B. {option_2}
C. {option_3} D. {option_4}

参考知识：
{knowledge}

只输出正确选项的完整文本，不要解释。
\end{PromptVerb}
\end{systemcard}

% =============================================================================
\subsection{Plan-Act-Replan Agent with LangGraph}
\label{app:par_agent}

\paragraph{System description.}
Plan-Act-Replan runs search as an explicit loop. Each round, the planner is given the image, question, options, the evidence gathered so far, and a record of past tool calls. It judges whether the current evidence is sufficient for answering. If not, it selects one retrieval tool and prepares the corresponding tool input. The environment executes the tool call, adds the returned observation to the evidence pool, and passes control back to the planner.

\begin{algorithm}[H]
\caption{Plan-Act-Replan Agent}
\label{alg:appendix_par}
\begin{algorithmic}[1]
\Require question $q$, options $O$, image $I$, maximum rounds $R$, retrieval depth $k$
\Ensure predicted answer $a^*$

\State $\mathcal{E} \leftarrow \emptyset$
\Comment{evidence pool}
\State $\mathcal{U} \leftarrow \emptyset$
\Comment{used tools}
\State $\mathcal{H} \leftarrow \emptyset$
\Comment{tool-call history}

\For{$r=1$ \textbf{to} $R$}
    \State $d \leftarrow
    \mathrm{LLM}_{\mathrm{plan}}(I,q,O,\mathcal{E},\mathcal{U},\mathcal{H},r)$
    \Comment{$d$ contains \field{can\_answer\_now}, \field{selected\_tool}, \field{bm25\_query}, reason, and confidence}

    \If{$d.\mathrm{can\_answer\_now}=\mathrm{true}$ \textbf{or}
    $d.\mathrm{selected\_tool}=\tool{none}$}
        \State \textbf{break}
    \EndIf

    \State $\tau \leftarrow d.\mathrm{selected\_tool}$

    \If{$\tau=\tool{bm25\_ann}$}
        \State $\mathrm{query} \leftarrow d.\mathrm{bm25\_query}$
        \Comment{planner-generated keyword query}
    \ElsIf{$\tau=\tool{img\_ann}$}
        \State $\mathrm{query} \leftarrow I$
    \ElsIf{$\tau=\tool{text\_ann}$}
        \State $\mathrm{query} \leftarrow q$
    \Else
        \State $\mathrm{query} \leftarrow (I,q)$
        \Comment{\tool{multimodal\_ann}}
    \EndIf

    \State $\mathcal{R} \leftarrow \mathrm{ANN}_{\tau}(\mathrm{query},k)$
    \State $\mathcal{E} \leftarrow \mathcal{E} \cup \mathrm{ExtractTopK}(\mathcal{R})$
    \State $\mathcal{U} \leftarrow \mathcal{U} \cup \{\tau\}$
    \State $\mathcal{H} \leftarrow
    \mathcal{H} \cup \{(\tau,|\mathcal{R}|,\mathrm{error}(\mathcal{R}))\}$

    \If{$\tau=\tool{img\_ann}$ \textbf{and} $\mathcal{R}\neq\emptyset$}
        \State $Q_{\mathrm{kn}} \leftarrow
        \mathrm{MajorityVote}(\{r.\mathrm{query}\mid r\in\mathcal{R}\})$
        \State $\mathcal{K} \leftarrow \mathrm{KnLookup}(Q_{\mathrm{kn}})$
        \If{$\mathcal{K}\neq\emptyset$}
            \State $\mathcal{E} \leftarrow \mathcal{E} \cup \mathcal{K}$
        \EndIf
    \EndIf
\EndFor

\State $a^* \leftarrow \mathrm{LLM}_{\mathrm{answer}}(I,q,O,\mathcal{E})$
\State \Return $a^*$
\end{algorithmic}
\end{algorithm}

\paragraph{Tool skill cards.}
The planner is guided by skill cards that define each tool's use cases, request schema, response fields, and decision hints. The original cards are included below.

\begin{systemcard}{gaLightBlue}
\cardtitle{gaBlue}{SKILL.md: ann-bm25-recall}
\begin{PromptVerb}
---
name: ann-bm25-recall
description: BM25 keyword retrieval tool skill. Use when the question contains specific names, terms or IDs that should be matched exactly in the knowledge base, and semantic embedding may miss them.

---

# ann-bm25-recall

## Tool Name

`bm25_ann`

## When to use

- 题目包含**专有名词、角色名、技能名、地图名、道具名**等需要精确匹配的关键词。
- 语义向量召回（`text_ann` / `multimodal_ann`）结果不相关，或分数偏低时。
- 你希望用**关键词组合**直接锁定知识片段，而非依赖语义相似度。
- 图像已能确认某个具体名称，但仍需其文字描述或规则说明。

## 特别说明：query 由大模型生成

与其他 ANN 工具直接使用原始问题作为查询不同，`bm25_ann` 的查询由 **planner 在规划时
生成**，写入 `bm25_query` 字段。  
Query 应是**简短的关键词组合**，而非完整问句，例如：

| 原始问题                           | 好的 bm25_query               |
| ---------------------------------- | ----------------------------- |
| 原神中雷电将军的终结技叫什么名字？ | `原神 雷电将军 终结技 名称`   |
| 火影忍者手游里鸣人有哪些觉醒？     | `火影忍者手游 漩涡鸣人 觉醒`  |
| CS:GO Dust II 的A点炸弹区在哪里？  | `CS:GO Dust2 A点 炸弹区 位置` |

## Request

- Method: `POST`
- Endpoint: `/bm25_ann`
- JSON payload:

```json
{
  "query": "原神 雷电将军 终结技 名称",
  "top_k": 5
}
```

> `query` 填入 planner 生成的 `bm25_query`，而非原始问题。

## Response

- 读取 `scores` 字段作为召回结果列表。
- 常见字段：`title`、`content`、`chunk_id`、`score`（BM25 分数，越高越相关）。
- 若所有文档均无词语重叠，`scores` 为空列表。

## Decision Hints

- 若问题核心是**精确关键词命中**，优先本工具。
- 若问题需要**语义相似度**或**跨语言理解**，优先 `text_ann` 或 `multimodal_ann`。
- 本工具与 `text_ann` 互补：两者同时用可提升召回覆盖度。
  \end{PromptVerb}
  \end{systemcard}

\begin{systemcard}{gaLightBlue}
\cardtitle{gaBlue}{SKILL.md: ann-image-recall}
\begin{PromptVerb}
---
name: ann-image-recall
description: Image ANN retrieval tool skill. Use when the answer depends on visual similarity, UI style, iconography, or scene details from the image.

---

# ann-image-recall

## Tool Name

`img_ann`

## When to use

- 题目与图像中的视觉元素高度相关（界面样式、图标、角色外观、场景布局）。
- 需要在图库中找“视觉上最像”的样本作为参考。
- 文本召回不足以解释图像细节。

## Request

- Method: `POST`
- Endpoint: `/img_ann`
- JSON payload:

```json
{
  "img": "/path/to/image.jpg",
  "top_k": 5
}
```

## Response

- 读取 `scores` 字段作为召回结果列表。
- 常见字段：`img`、`query`、`pid`、`score`。

## Knowledge Enrichment（自动触发，无需额外规划）

调用 `img_ann` 后，pipeline 会自动执行以下步骤：

1. 从召回 top-N 结果中提取每条记录的 `query` 字段（该字段为与图库图片关联的知识查询文本）。
2. 通过策略（众数投票或 LLM 相关性判断）选出最有价值的 query。
3. 调用内部 `kn_lookup` 服务，检索对应详细知识内容（游戏地图介绍、武器说明、规则解释等）。
4. 将知识内容追加至证据，供答题器使用。

因此，`img_ann` 不仅返回视觉相似图像，**还会自动补充相关知识文本**。

## Decision Hints

- 当”看图找相似”是主需求时优先本工具。
- 若题目同时依赖文本语义和图像语义，可优先尝试 `multimodal_ann`。
- 当题目涉及游戏机制、地图规则、武器参数等知识型内容，且图像有明确游戏/场景标识时，`img_ann` + 自动知识补充的组合效果更优。
  \end{PromptVerb}
  \end{systemcard}

\begin{systemcard}{gaLightBlue}
\cardtitle{gaBlue}{SKILL.md: ann-multimodal-recall}
\begin{PromptVerb}
---
name: ann-multimodal-recall
description: Multimodal ANN retrieval tool skill. Use when both text intent and image evidence are needed together to recall the most relevant knowledge.

---

# ann-multimodal-recall

## Tool Name

`multimodal_ann`

## When to use

- 问题需要同时结合“图像内容 + 查询文本”才能准确检索。
- 单独文本 ANN 或图像 ANN 的结果都不稳定时。
- 你希望一次召回就兼顾语义和视觉相关性。

## Request

- Method: `POST`
- Endpoint: `/multimodal_ann`
- JSON payload:

```json
{
  "query": "天涯明月刀 一代宗师毒圈 基本规则",
  "image_path": "/path/to/image.jpg",
  "top_k": 5
}
```

## Response

- 读取 `scores` 字段作为召回结果列表。
- 常见字段：`title`、`content`、`source_query`、`source_best_img`、`score`。

## Decision Hints

- 当你不确定该选文本还是图像召回时，优先尝试本工具。
- 若仍无法回答，可再补一个 `text_ann` 或 `img_ann`。
  \end{PromptVerb}
  \end{systemcard}

\newpage
\begin{systemcard}{gaLightBlue}
\cardtitle{gaBlue}{SKILL.md: ann-text-recall}
\begin{PromptVerb}
---
name: ann-text-recall
description: Text ANN retrieval tool skill. Use when the question needs external textual knowledge, concept definitions, or rule details not directly visible in the image.

---

# ann-text-recall

## Tool Name

`text_ann`

## When to use

- 题目主要是概念、机制、背景知识，图像本身无法直接给出完整答案。
- 需要通过文本语义找相近知识片段（如术语解释、规则描述）。
- 你已经看过图像，但仍存在明显知识缺口。

## Request

- Method: `POST`
- Endpoint: `/text_ann`
- JSON payload:

```json
{
  "query": "天涯明月刀 一代宗师毒圈 基本规则",
  "top_k": 5
}
```

## Response

- 读取 `scores` 字段作为召回结果列表。
- 常见字段：`title`、`content`、`score`、`chunk_id`。

## Decision Hints

- 若问题核心是“文本知识匹配”，优先尝试本工具。
- 若问题核心是“画面视觉细节”，优先考虑 `img_ann` 或 `multimodal_ann`。
  \end{PromptVerb}
  \end{systemcard}

\begin{systemcard}{gaLightBlue}
\cardtitle{gaBlue}{SKILL.md: kn-lookup}
\begin{PromptVerb}
---
name: kn-lookup
description: Knowledge base lookup service. Given a list of query strings (obtained from img_ann results), returns the corresponding long-form knowledge content from the internal knowledge base. This service is automatically triggered after img_ann and does not need to be called manually by the planner.
---

# kn-lookup

## Overview

`kn_lookup` 是一个本地知识库查询服务。它根据图像召回（`img_ann`）返回的 `query` 字段，在预构建的知识字典中检索对应的详细文本内容（如游戏规则、地图介绍、武器说明等）。

该服务在 `img_ann` 调用后**自动触发**，不需要规划器单独决策调用。
---
## 工作流程
```
img_ann 召回 → 提取 top-N query → 策略选取 → kn_lookup → 知识内容追加到证据
```
1. `img_ann` 返回 `records`，每条记录含 `query` 字段（与图库图片关联的文本查询）。
2. 从 top-N 记录中提取 `query`，通过策略（众数投票 / LLM 相关性判断）选出最有价值的查询。
3. 调用 `kn_lookup` 服务，查出对应的知识内容。
4. 将知识内容拼入证据（`evidence`）中，供答题器参考。

---
## Request

- Method: `POST`
- Endpoint: `/kn_lookup`
- JSON payload:

```json
{
  "queries": ["CS:GO Dust II", "CS:GO Mirage"]
}
```

| 字段      | 类型        | 说明                                                         |
| --------- | ----------- | ------------------------------------------------------------ |
| `queries` | `list[str]` | 要查询的 query 字符串列表，来自 `img_ann` records 的 `query` 字段 |

---
## Response

```json
{
  "results": [
    {
      "query": "CS:GO Dust II",
      "found": true,
      "contents": [
        "### 游戏内容介绍：CS:GO Dust II\n\n...",
        "在CS:GO地图Dust II中，..."
      ]
    },
    {
      "query": "CS:GO Unknown Map",
      "found": false,
      "contents": []
    }
  ]
}
```

| 字段       | 说明                                                         |
| ---------- | ------------------------------------------------------------ |
| `found`    | 是否在知识库中找到该 query                                   |
| `contents` | 匹配的知识内容列表（同一 query 在两个文件中均有时，返回两条） |

---
## Query 选取策略

### 众数投票（默认，`majority`）

统计 `img_ann` top-N 结果中各 query 出现次数，选出频率最高的 K 个 query 进行知识查询。

- 优点：零额外 LLM 开销，快速稳定。
- 适用：图像库中同一主题出现频繁时（如同一游戏地图有多张截图）。

### LLM 相关性选取（`llm`）

将所有候选 query 连同当前题目发给 LLM，由 LLM 判断哪些 query 对解题最有帮助，输出选中的 query 列表。

- 优点：能结合题意做语义对齐，精度更高。
- 适用：图像库 query 多样，需要语义判断时。

---
## 服务启动

```bash
python tools/kn_lookup_server.py          # 默认端口 8002
KN_PORT=9002 python tools/kn_lookup_server.py
KN_FILES=tools/query_rag_kn_part_1.jsonl:tools/qwen_rag_kn_part_2.jsonl python tools/kn_lookup_server.py
```

## 健康检查

```
GET /health
→ {"status": "ok", "num_unique_queries": 22800}
```

## Decision Hints（供规划器参考）

- `kn_lookup` 由 pipeline 自动触发，无需规划器主动选择。
- 当 `img_ann` 证据中 `query` 字段有明确语义（如游戏名称、地图名、武器名）时，知识库极有可能命中，补充知识效果显著。
- 若知识库未命中（`found=false`），不影响其他证据正常使用。
  \end{PromptVerb}
  \end{systemcard}

% =============================================================================
\subsection{MMSearch-R1 Agentic-RL Search Model}
\label{app:msr1_agent}

\paragraph{System description.}
MS-R1 internalizes tool use into model generation. Instead of relying on an external planner, the model first generates reasoning and then emits either a final-answer tag or a tool-call tag. The environment parses the action, executes the corresponding retrieval tool, appends the returned observation, and continues the generation process.

\begin{algorithm}[H]
\caption{MS-R1 Search Inference and GRPO Training}
\label{alg:appendix_msr1}
\begin{algorithmic}[1]
\Require image $I$, question $q$, options $O$, policy $\pi_\theta$,
reference policy $\pi_{\mathrm{ref}}$, retrieval depth $k$, mode
$m \in \{\textsc{Infer},\textsc{Train}\}$
\Ensure answer $a^*$ if $m=\textsc{Infer}$; updated policy $\pi_\theta$ if $m=\textsc{Train}$

\Statex \textbf{Shared three-round search rollout.}
\Function{Rollout}{$\pi, I, q, O, k, \mathrm{decode}$}
    \State Initialize context $c_1$ with $(I,q,O)$ and the round-1 prompt;
    initialize trajectory $\tau \leftarrow \emptyset$
    \For{$t=1$ \textbf{to} $3$}
        \State Generate $y_t \sim \pi(\cdot \mid c_t)$ using $\mathrm{decode}$;
        append $y_t$ to $\tau$
        \State $(\alpha_t, z_t) \leftarrow \mathrm{ParseAction}(y_t)$
        \Comment{$\alpha_t \in \{\textsc{Answer},\textsc{ImageSearch},\textsc{TextSearch},\textsc{Invalid}\}$}
        \If{$\alpha_t=\textsc{Answer}$ \textbf{or} $t=3$}
            \State $a \leftarrow \mathrm{ExtractAnswer}(y_t)$;
            \Return $(a,\tau)$
        \ElsIf{$\alpha_t \in \{\textsc{ImageSearch},\textsc{TextSearch}\}$}
            \State $(o_t, p_t) \leftarrow \mathrm{ExecuteTool}(\alpha_t,z_t,I,k)$
            \Comment{return observation and next-stage prompt}
            \State $c_{t+1} \leftarrow c_t \oplus y_t \oplus o_t \oplus p_t$;
            append $o_t$ to $\tau$
        \Else
            \State Mark $y_t$ as invalid in $\tau$
        \EndIf
    \EndFor
\EndFunction

\Statex\vspace{2pt}
\Statex \textbf{Inference.}
\If{$m=\textsc{Infer}$}
    \State $(a^*,\tau) \leftarrow \Call{Rollout}{\pi_\theta,I,q,O,k,\mathrm{greedy}}$
    \State \Return $a^*$
\EndIf

\Statex\vspace{2pt}
\Statex \textbf{Training.}
\State Sample $G$ trajectories
$\{(a_i,\tau_i)\}_{i=1}^{G}$ by
$\Call{Rollout}{\pi_\theta,I,q,O,k,\mathrm{sample}}$
\State $R_i \leftarrow R_{\mathrm{ans}}(a_i)
+ R_{\mathrm{format}}(\tau_i)
+ R_{\mathrm{tool}}(\tau_i)$ for each trajectory $i$
\State Normalize $\{R_i\}_{i=1}^{G}$ within the group to obtain advantages $\{A_i\}_{i=1}^{G}$
\State Update $\pi_\theta$ with GRPO using $\{(\tau_i,A_i)\}_{i=1}^{G}$ and KL regularization to $\pi_{\mathrm{ref}}$
\State \Return $\pi_\theta$
\end{algorithmic}
\end{algorithm}

\paragraph{Rollout and reward.}
\textsc{ImageSearch} and \textsc{TextSearch} are parsed from
\tagtok{<search><img>} \tagtok{</search>} and
\tagtok{<text\_search>...</text\_search>}. $\mathrm{ExecuteTool}$ calls
\tool{img\_ann} or \tool{text\_ann}, wraps the result in
\tagtok{<information>...</information>}, and appends the next-stage prompt.
Inference uses one greedy rollout, while training samples trajectories in groups and applies GRPO. The reward combines answer correctness, format validity, and tool-call validity, with a KL penalty against the reference model.

\paragraph{Prompt templates.}
Three stage-specific prompt templates define the MS-R1 interaction process. The first prompt defines the allowed actions and the three-round interaction constraint. The second prompt is used after image search and asks the model to determine whether the image-search observation is sufficient or whether text search is needed. The third prompt is used after text search and requires the model to produce the final answer. The original Chinese prompt templates are included below.

\begin{systemcard}{gaLightOrange}
\cardtitle{gaOrange}{round1 user prompt}
\begin{PromptVerb}
请根据给定图片回答用户问题。你正在参与一个多轮推理任务，允许你在必要时先调用搜索工具，再在后续轮次继续作答。

你需要遵循以下总体原则：

* 你的输出必须始终先写在 <reason>...</reason> 中，再决定下一步动作。
* 合法动作只有三种：

  1. 直接给出最终答案：<answer>...</answer>
  2. 调用图搜工具：<search><img></search>
  3. 调用文本搜索工具：<text_search>你的查询</text_search>
* 最终答案必须放在 <answer>...</answer> 中，答案要简洁明确，不要展开解释。
* 如果题目给了多个候选答案，你在最终答案中必须输出完整的候选内容本身，不要输出缩写、简称、编号、代号，也不要只输出部分关键词。

你可能出现的合法链路包括：

1. 单轮：直接回答。
2. 双轮：先图搜，再回答。
3. 双轮：先文搜，再回答。
4. 三轮：先图搜，再文搜，最后回答。

请按下面顺序决策：

1. 先判断这个问题是否真的依赖图片。如果问题主要依赖常识或文本知识，而图片不是关键证据，则可以直接回答。
2. 如果问题依赖图片，再判断当前图片是否已经足够让你确认与问题相关的核心游戏元素。
3. 只要你对关键游戏元素、名称、物品、角色、地点、机制、界面名词或其他核心实体不是特别确定，或者虽然看出一些线索但还不能稳定支撑答案，就优先调用图搜工具，在回复末尾输出 <search><img></search>。不要因为勉强猜到一个可能答案就跳过图搜。
4. 对于明显依赖图片的问题，只要你还不能非常稳定地说出“这张图里最关键的元素到底是什么”，默认优先图搜通常比直接猜更稳妥。与其冒险直接回答，不如先通过图搜确认元素。
5. 图搜的核心作用通常不是直接给出最终答案，而是帮助你确认图片对应的游戏元素、名称、物品、角色、地点、机制、界面名词或其他关键实体。
6. 一旦你已经确认了最可能的游戏元素，就判断是否已经可以结合你的已有知识直接回答。如果仍然不能稳定回答，就必须基于“游戏元素 + 用户问题”构造一个简洁、具体、可检索的文本搜索 query，并在回复末尾输出 <text_search>你的查询</text_search>。

请特别注意：

* 对依赖图片的问题，图搜通常是一个值得优先尝试的步骤；如果你还在犹豫是否已经认准了元素，优先图搜通常比直接猜更稳妥。
* 即使你已经隐约猜到某个答案，只要关键视觉元素还没有确认清楚，仍然应该优先图搜，而不是直接凭印象作答。
* 图搜结果通常只是帮助你确认“这是哪个游戏元素”，后续真正关键的是利用这个元素信息继续推理。
* 搜索结果可能存在噪声、误召回或不完整信息，不要机械相信返回内容；你必须结合原图、用户问题、搜索分数和已有知识判断其是否可信。也就是说，可以先搜，再决定是否采用搜索结果。
* 如果图搜结果里至少有部分候选与原图足够接近，这些结果就值得拿来帮助你缩小元素范围，而不是因为存在误召回就完全放弃搜索结果。
* 如果需要做文本搜索，query 中不要遗漏已经确认的游戏元素名称，这是检索到正确信息的关键。
* 如果题目给了多个候选内容，你应输出你认为正确的那个候选内容的完整文本，不要偷懒省略成简短代称。
* 不要同时输出多个动作。
* 当你准备输出最终答案时，不要再调用任何工具。
* 示例：<answer>Titanic</answer>

所有后续搜索结果都会放在 <information>...</information> 中返回给你。

下面是图片与问题： <image>

问题：
{question}

候选答案：
{options}

请从给定候选答案中选择最正确的一项。请注意：如果你最终作答，必须输出完整候选答案内容本身，不要输出编号、字母、简称或部分片段。

额外约束：整个任务中，模型最多只能进行 3 次回复（即最多 3 轮 assistant 输出）。如果你已经进入第 3 次回复，就必须直接给出最终答案，不能再调用任何搜索工具。
\end{PromptVerb}
\end{systemcard}

\newpage
\begin{systemcard}{gaLightOrange}
\cardtitle{gaOrange}{after image search prompt}
\begin{PromptVerb}
你已经完成了一轮图搜。现在你处于多轮任务的中间阶段，需要根据图搜结果决定：是直接回答，还是继续进行文本搜索。

你仍然必须遵守统一格式：
* 先在 <reason>...</reason> 中进行分析。
* 然后只能选择以下两种动作之一：
  1. 直接回答：<answer>...</answer>
  2. 继续文本搜索：<text_search>你的查询</text_search>

请按下面顺序思考：
1. 先结合原图、用户问题以及图搜返回的多个候选结果，判断原图最对应的核心游戏元素是什么。
2. 重点参考返回结果中的元素名称、标题、关键词和分数，同时结合图搜返回的图片与原始 query 图片进行比对，判断哪个候选在视觉上和语义上都最匹配当前问题。图搜图片的核心价值是帮助你确认元素信息。
3. 注意，图搜结果可能存在误召回，分数高只表示相对更相似，不等于一定正确。你需要检查返回图片中的角色、物体、场景、UI、文本或关键元素是否真的与原图一致或足够接近；如果不一致，就应降低对该结果的信任。
4. 你可以把分数当作一个较强但不是绝对的参考：
   * 如果某个候选分数大于 0.95，并且视觉上与原图关键元素基本一致，通常可以较高置信地采信。
   * 如果某个候选分数大于 0.90，通常说明它比较可信，但仍要结合原图中的关键细节再确认。
   * 如果候选分数小于 0.90，就要更加仔细辨别；除非视觉证据非常吻合，否则一般不要轻易相信。
5. 即使图搜没有直接给出答案，它仍然可能帮助你缩小元素范围。你需要先判断哪些结果可采信、哪些结果应忽略，而不是直接照单全收。
6. 如果图搜结果里有一个或几个候选与原图明显更接近，你应优先把这些候选当作后续推理的基础，而不是继续停留在模糊猜测上。
7. 一旦确认了最可能的游戏元素，就判断：仅凭这个元素提示和你已有的知识，是否已经足以回答用户问题。
8. 如果已经足够回答，就直接给出最终答案。
9. 如果仍然不能稳定回答，就必须围绕“已确认的游戏元素 + 用户问题”构造一个高质量文本搜索 query，并在回复末尾输出 <text_search>你的查询</text_search>。

请特别注意：
* 图搜通常不能直接给出最终答案，它更重要的作用是帮助你确认原图对应的元素信息。
* 如果图搜结果彼此接近，你应在 <reason> 中说明你为何选择某个元素作为后续推理基础，尤其要说明它与原图、当前问题和图搜分数的匹配依据。
* 如果图搜结果整体都不可信，不要把误召回结果当成事实；但只要某些结果能帮助你进一步锁定元素范围，就可以据此继续做更有针对性的文本搜索。
* 当你对元素已经有一定把握，但对题目中的具体机制、数值、条件或隐藏规则还不够确定时，优先继续文本搜索，而不是仓促直接回答。
* 文本搜索 query 不能只重复用户原问题，必须显式包含你确认出的游戏元素名称或核心实体，这是文本搜索成功的关键。
* 如果题目给了多个候选内容，最终答案必须写出完整候选内容本身，不要输出缩写、代号或部分片段。
* 这一轮不要再调用图搜。
* 如果给出最终答案，必须使用 <answer>...</answer> 包裹，且答案保持简洁。
* 示例：<answer>Titanic</answer>

额外约束：这通常是任务的第 2 次回复。如果你此时选择继续文本搜索，那么下一次回复必须直接输出最终答案，不能再调用任何工具。
\end{PromptVerb}
\end{systemcard}

\begin{systemcard}{gaLightOrange}
\cardtitle{gaOrange}{after text search prompt}
\begin{PromptVerb}
你已经完成文本搜索，现在处于多轮任务的最后收束阶段。此时你的目标是结合已有信息，尽可能稳定地给出最终答案。
你仍然必须遵守统一格式：
* 先在 <reason>...</reason> 中分析。
* 然后输出最终答案：<answer>...</answer>

请结合以下信息完成最终推理：
* 用户原问题
* 之前确认出的游戏元素或核心实体
* 当前返回的文本搜索结果

要求如下：
1. 在 <reason> 中说明文本搜索结果如何支持某个答案，以及你如何利用前面确认的游戏元素缩小范围。
2. 文本搜索结果也可能包含噪声、错页、泛化描述或与当前元素不完全对应的内容。你需要优先采信与已确认游戏元素、问题语义和候选答案都一致的结果，而不是机械相信任意一条检索信息。
3. 如果文本搜索结果与前面确认的游戏元素明显不一致，或者只支持了一个过于泛化的结论，你应降低其权重，并结合上下文做更稳妥的判断。
4. 如果多条检索结果彼此冲突，你应优先采用与已确认元素更一致、与问题更贴合、且能更直接支持某个候选答案的证据。
5. 如果检索结果仍不完全充分，也要结合你已有知识和上下文，选择当前最合理、最恰当的答案。
6. 如果题目给了多个候选内容，最终答案必须输出完整候选内容本身，不要输出缩写、代号、部分关键词或不完整片段。
7. 不要输出拒答语句，也不要继续调用任何工具。
8. 最终答案必须放在 <answer>...</answer> 中，答案要简洁、明确，不要额外展开。

请记住：文本搜索阶段的核心不是重新泛化问题，而是利用前面已经确认的游戏元素与检索结果完成收束并最终回答。
额外约束：这已经是最后收束阶段，通常对应任务中的最后一次回复。你这一轮必须直接输出最终答案，不能继续搜索，也不能输出额外的下一步计划。
\end{PromptVerb}
\end{systemcard}

% =============================================================================
\subsection{Paradigm Comparison}
\label{app:paradigm_comparison}

The three tool-augmented settings differ in their level of search autonomy
rather than in the retrieval resources they can access. Fixed RAG follows a
hard-coded image-to-text retrieval chain and serves as a simple reproducible
baseline. PAR exposes the same tools to an explicit planner, allowing the model
to adaptively choose between visual, semantic, lexical, and multimodal retrieval.
MS-R1 further internalizes tool invocation into the model generation process
and learns search behavior through outcome-based reinforcement learning.

Table~\ref{tab:appendix_retrieval_interfaces} summarizes the shared retrieval
tools used by these settings. Since the tool set is fixed across methods,
performance differences mainly reflect search behavior, tool-use planning,
and evidence integration under controlled retrieval conditions.

\begin{table}[htbp]
\centering
\small
\setlength{\tabcolsep}{4pt}
\caption{Shared retrieval tools used across the three tool-augmented settings.}
\label{tab:appendix_retrieval_interfaces}
\begin{tabular}{p{0.17\linewidth} p{0.19\linewidth} p{0.56\linewidth}}
\toprule
\textbf{Tool} & \textbf{Input} & \textbf{Function} \\
\midrule
\tool{img\_ann}
& Image
& Retrieves visually similar game images from the frozen image pool. Each
retrieved record is associated with a core-element query, enabling downstream
knowledge lookup. \\

\tool{text\_ann}
& Text query
& Retrieves semantically relevant knowledge chunks from the text index. It is
used for game rules, concept definitions, equipment effects, background descriptions,
and mechanics. \\

\tool{bm25\_ann}
& Keyword query
& Performs sparse lexical retrieval over the knowledge chunks. It is useful for
exact matching of character names, map names, skill names, equipment names,
interface terms, and other game-specific entities. \\

\tool{multimodal\_ann}
& Image and text query
& Retrieves evidence using both visual content and textual intent. It is used
when neither image-only nor text-only retrieval is sufficient. \\

\tool{kn\_lookup}
& Core-element query
& Looks up structured knowledge associated with a core element. It is
automatically triggered after \tool{img\_ann} and is not exposed as an
independent planner action. \\
\bottomrule
\end{tabular}
\end{table}
