# Supplementary material for: SVFSearch: A Multimodal Knowledge-Intensive Benchmark for Short-Video Frame Search in the Gaming Vertical Domain
Source: arXiv:2605.17946 source file (2026-05-20)
Supplement: Supplementary file 4 [file D.case_show.tex]

% ---------- Theme palette ----------
\definecolor{cardbg}{HTML}{F5F6F8}
\definecolor{cardborder}{HTML}{D8DCE3}
\definecolor{accentBlue}{HTML}{3B6FB6}     % video info
\definecolor{accentTeal}{HTML}{2E8B8B}     % query
\definecolor{accentGray}{HTML}{6B7280}     % vanilla model
\definecolor{accentPurple}{HTML}{7C3AED}   % thinking model
\definecolor{accentBrown}{HTML}{92400E}    % RAG（赭石棕）
\definecolor{accentOrange}{HTML}{D97706}   % langgraph
\definecolor{accentGreen}{HTML}{059669}    % MMSearch-R1
\definecolor{correctRed}{HTML}{C0392B}
\definecolor{labelGray}{HTML}{4B5563}
\definecolor{enText}{HTML}{555555}

% ---------- Custom commands ----------
% Correct answer highlighting
\newcommand{\correct}[1]{\textcolor{correctRed}{\textbf{#1}}}
 
% Bilingual line: \bi{中文}{English}
\newcommand{\bi}[2]{%
  #1\\[1pt]%
  {\small\itshape\color{enText}#2}%
}
 
% Section label inside a card
\newcommand{\fieldlabel}[1]{{\footnotesize\bfseries\color{labelGray}#1}}
 
% ---------- Outer showcase wrapper ----------
\newtcolorbox{showcasebox}[1][]{
  enhanced,
  breakable,
  colback=white,
  colframe=cardborder,
  boxrule=0.6pt,
  arc=4pt,
  before skip=0pt,
  after skip=6pt,
  left=10pt, right=10pt, top=8pt, bottom=8pt,
  title=#1,
  fonttitle=\bfseries\small\color{white},
  colbacktitle=labelGray,
  attach boxed title to top left={xshift=8pt, yshift=-4pt},
  boxed title style={
    colframe=labelGray, arc=2pt, boxrule=0pt,
    left=6pt, right=6pt, top=2pt, bottom=2pt,
  },
}
 
% ---------- Section sub-card (video info / query) ----------
\newtcolorbox{subcard}[2]{
  enhanced,
  breakable,
  colback=cardbg,
  colframe=#1,
  boxrule=0pt,
  leftrule=3pt,
  arc=2pt,
  left=10pt, right=10pt, top=6pt, bottom=6pt,
  title=\textbf{\small\color{#1}#2},
  fonttitle=\normalfont,
  coltitle=#1,
  colbacktitle=cardbg,
  attach title to upper,
  after title={\par\vspace{4pt}},
}
 
% ---------- Model output card ----------
% Args: {accent color}{model name}{verdict icon+text}
\newtcolorbox{modelcard}[3]{
  enhanced,
  breakable,
  colback=cardbg,
  colframe=#1,
  boxrule=0pt,
  leftrule=3pt,
  arc=2pt,
  left=10pt, right=10pt, top=3pt, bottom=3pt,
  title={\textbf{\small\color{#1}#2}\hfill{\small #3}},
  fonttitle=\normalfont,
  coltitle=#1,
  colbacktitle=cardbg,
  attach title to upper,
  after title={\par\vspace{4pt}},
}
 
% Verdict icons
\newcommand{\verdictCorrect}{\textcolor{accentGreen}{\faCheckCircle\ \textbf{Correct}}}
\newcommand{\verdictWrong}{\textcolor{correctRed}{\faTimesCircle\ \textbf{Wrong}}}
 
% Multiple-choice option list
\newenvironment{choices}{%
  \begin{list}{}{%
    \setlength{\leftmargin}{1.2em}%
    \setlength{\itemsep}{1pt}%
    \setlength{\parsep}{0pt}%
    \setlength{\topsep}{2pt}%
  }%
}{\end{list}}
\newcommand{\choice}[2]{\item[\textbf{#1.}] #2}
 
% ---------- Retrieval reference (Style D) ----------
% Inline reference token in reasoning text, e.g. \refTag{R1}
% Renders as a small pill: [R1] in monospace, light blue background.
\definecolor{refBg}{HTML}{E8F0F8}
\definecolor{refBorder}{HTML}{C8D8E8}
\definecolor{refText}{HTML}{1F4E79}
\newcommand{\refTag}[1]{%
  \tikz[baseline=(r.base)]\node[
    inner xsep=3pt, inner ysep=0.5pt,
    rounded corners=1.2pt,
    fill=refBg, draw=refBorder, line width=0.3pt,
    font=\ttfamily\footnotesize\bfseries\color{refText}
  ] (r) {[#1]};%
}
 
\newenvironment{retrievalGallery}{%
  \par\vspace{4pt}%
  {\color{cardborder}\rule{\linewidth}{0.4pt}}\par% dashed-look separator
  \vspace{2pt}%
  {\footnotesize\bfseries\color{labelGray}RETRIEVED EVIDENCE}\par
  \vspace{3pt}%
  \noindent\begin{minipage}{\linewidth}\centering
}{%
  \end{minipage}\par
}
% \retrievalItem{label}{image path}{Chinese query}{English query}

% 图搜 item（带图，宽版）—— 顶部对齐
\newcommand{\retrievalItemImg}[4]{%
  \begin{minipage}[t]{0.46\linewidth}%
    \centering
    {\centering\refTag{#1}\par}%
    \vspace{2pt}%
    \includegraphics[width=0.85\linewidth, height=2.2cm, keepaspectratio]{#2}\\[4pt]
    \vspace{2pt}%
    {\footnotesize #3}\\
    {\scriptsize\itshape\color{enText}#4}
  \end{minipage}\hfill
}

% 文搜 item（纯文本）—— 顶部对齐
\newcommand{\retrievalItemText}[3]{%
  \begin{minipage}[t]{0.46\linewidth}%
    \refTag{#1}\\[2pt]
    {\footnotesize\bfseries\color{labelGray}QUERY:} {\footnotesize\itshape #2}\\[5pt]
    {\footnotesize\bfseries\color{labelGray}DOCUMENT:}\\[2pt]
    {\footnotesize #3}
  \end{minipage}\hfill
}

\newpage

\vspace{10em}
\section{Representative Examples}
\label{sec:representative_examples}
\vspace{-4em}
% ============================================================
%  CASE 1
% ============================================================
\begin{showcasebox}[Case 1]

% --- Video Information ---
\begin{subcard}{accentBlue}{\faVideo\ \ Video Information}

\fieldlabel{TITLE}\\[2pt]
\bi{鸣潮~鸣潮相里要~鸣潮吟霖~导电声骸速刷路线（1）}%
   {WutheringWaves XiangliYao Yinlin Electro (Conductive) Echo Farming Route (1)}

\vspace{6pt}
\fieldlabel{COVER OCR}\\[2pt]
\bi{导电套,彻空冥雷,COST3速刷路线,=C3}%
   {Electro Set – Void Thunder | COST 3 Speed Farming Route (C3)}

\vspace{6pt}
\fieldlabel{ASR TRANSCRIPT}\\[2pt]
\bi{大家好这里是霖宝，本期是导电声骸速刷路线。先传送到北落野信标，往右前方走，依次刷乐师、惊奇猎手；随后传送到燎照之骑全息左侧锚点，右转清理火属性怪、乐师和惊奇猎手。回头爬上高处，继续刷乐师和惊奇猎手……}%
   {Hi, this is Linbao. This is an Electro Echo farming route. First, teleport to the Beiluo Field waypoint, move to the front-right, and clear the Musician and Aberrant Hunters along the way. Then teleport to the waypoint left of the Inferno Rider Hologram, turn right, and clear the Fusion-type enemies, Musician, and Aberrant Hunters. Head back and climb up, then continue clearing more Musicians and Aberrant Hunters ...}

\end{subcard}

\vspace{6pt}

% --- Query ---
\begin{subcard}{accentTeal}{\faQuestionCircle\ \ Query}

\begin{center}
  \includegraphics[width=0.5\linewidth]{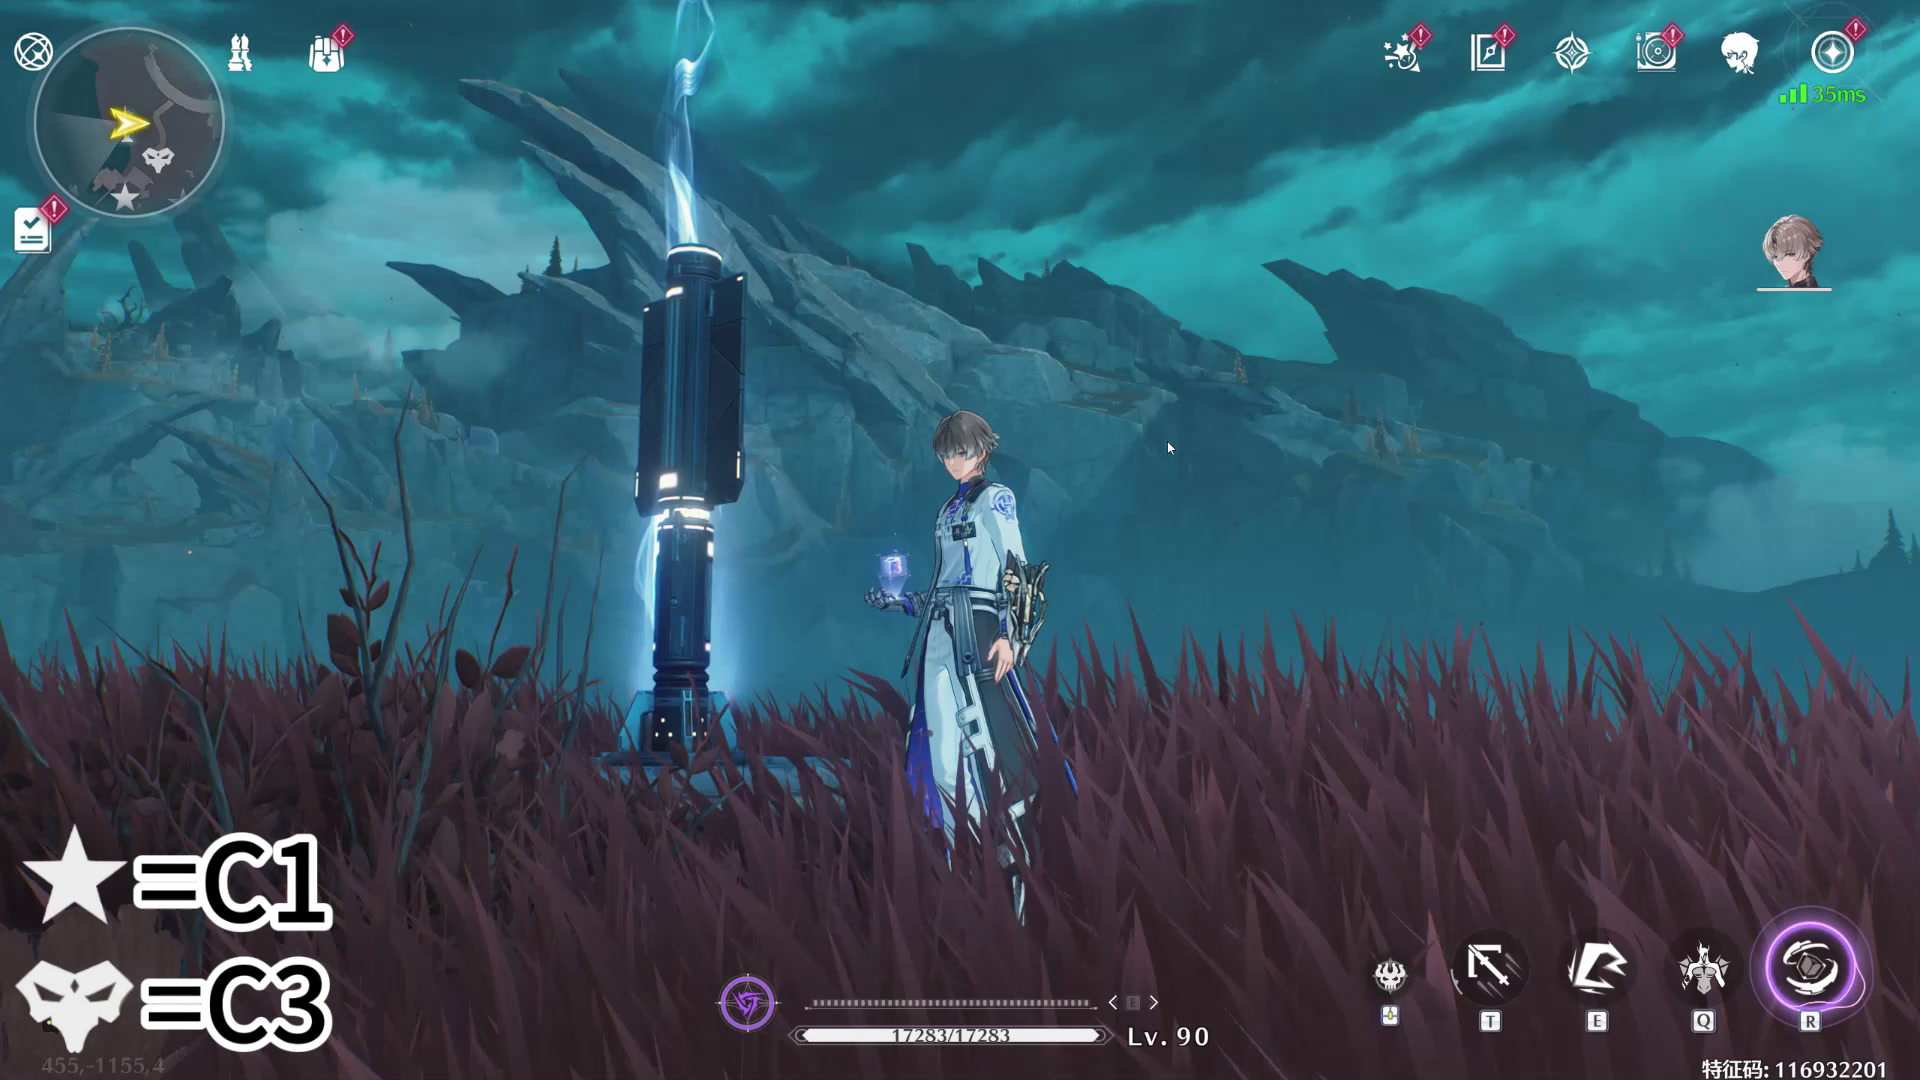}\\[2pt]
  {\footnotesize\itshape Query image}
\end{center}

\vspace{4pt}
\fieldlabel{QUESTION}\\[2pt]
\bi{该机制5件套效果最多可叠加几层导电伤害增益？}%
   {How many layers of conductive damage buff can this 5-piece set effect stack at most ?}

\vspace{6pt}
\fieldlabel{OPTIONS}\par
\vspace{2pt}

\noindent\hspace*{0.5em}%
\begin{minipage}{\dimexpr\linewidth-1.5em\relax}
\begin{choices}
  \choice{A}{\bi{1层}{1 stack}}
  \choice{B}{\correct{\bi{2层}{2 stacks}}}
  \choice{C}{\bi{3层}{3 stacks}}
  \choice{D}{\bi{4层}{4 stacks}}
\end{choices}
\end{minipage}

\vspace{4pt}
\fieldlabel{GROUND TRUTH}\ \ \correct{B. 2层\,/\,2 stacks}

\end{subcard}

\vspace{6pt}

% --- Model Outputs ---

\newpage

\noindent\textbf{\small Model Outputs}\\[0.5pt]

% Model 1: Vanilla
\begin{modelcard}{accentGray}{Vanilla Model}{\verdictWrong}
\fieldlabel{ANSWER:} C. 3 stacks

\vspace{1pt}
\end{modelcard}

\vspace{1pt}

% Model 2: Thinking
\begin{modelcard}{accentPurple}{Thinking Model}{\verdictWrong}
\fieldlabel{ANSWER:} C. 3 stacks

\vspace{1pt}
\fieldlabel{REASONING:} \textit{[Thinking]} The question asks for the maximum number of Electro DMG bonus stacks provided by the 5-piece set effect. The image mainly shows the game interface (character, skills, level), but no explicit evidence related to the stacking mechanic is present\ldots \\[2pt]
\textit{[Final]} Therefore, the most plausible answer is C. 3 stacks.
\end{modelcard}

\vspace{1pt}

% Model 3: RAG
\begin{modelcard}{accentBrown}{RAG (Ours)}{\verdictCorrect}
\fieldlabel{ANSWER:} \correct{B. 2 stacks}

\vspace{1pt}

\begin{retrievalGallery}
  \retrievalItemImg{R1}{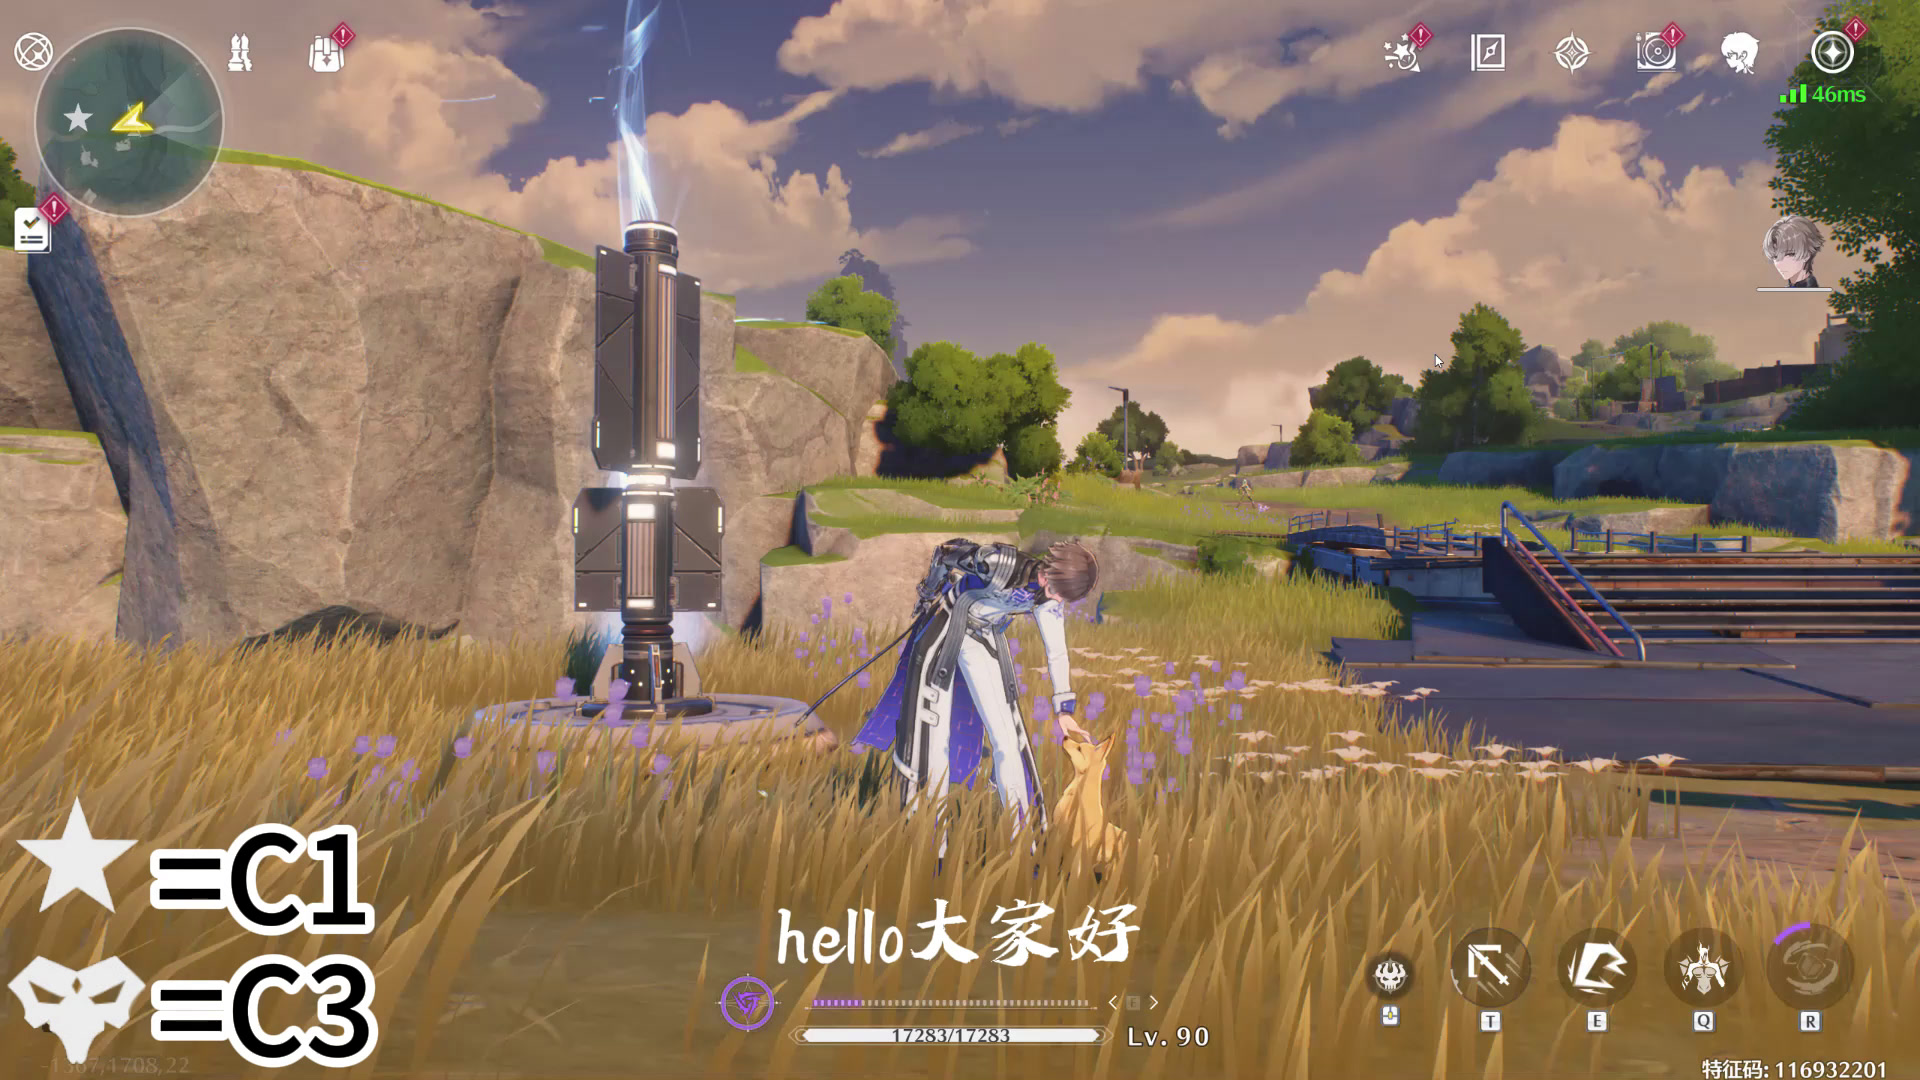}{鸣潮~合鸣·彻空冥雷}{Wuthering Waves Resonance: Void Thunder}
  \retrievalItemText{R2}%
    {In Wuthering Waves, under the Resonance: Void Thunder set, what is the maximum\ldots}%
    {Void Thunder (Wuthering Waves)\ldots 2-Piece: Electro DMG +10\%\ldots this effect can stack up to 2 times, with each stack lasting 15 seconds\ldots}
\end{retrievalGallery}
\end{modelcard}

\vspace{1pt}

% Model 4: LangGraph
\begin{modelcard}{accentOrange}{LangGraph (Ours)}{\verdictCorrect}
\fieldlabel{ANSWER:} \correct{B. 2 stacks}

\vspace{1pt}
\fieldlabel{REASONING:} 
\textit{[Plan]} Identify the set effect and its stacking rule…\\
\textit{[Tool: img\_ann]} Retrieve related image of “Resonance: Void Thunder” \ldots\\
\textit{[Tool: text\_ann]} Retrieve set description… result shows 5-piece effect grants Electro DMG bonus stacks\ldots\\
\textit{[Synthesize]} The description explicitly states the effect stacks up to 2 times, each lasting 15s\ldots thus answer is 2 stacks.

\begin{retrievalGallery}
  \retrievalItemImg{R1}{IMG/CASE_SHOW/CASE1/151565282692_001.jpg}{鸣潮~合鸣·彻空冥雷}{Wuthering Waves Resonance: Void Thunder}
  \retrievalItemText{R2}%
    {In Wuthering Waves, what is the max Electro DMG stacks from the 5-piece effect?}%
    {Void Thunder (Wuthering Waves)\ldots 2-Piece: Electro DMG +10\%\ldots this effect can stack up to 2 times, with each stack lasting 15 seconds\ldots}
\end{retrievalGallery}
\end{modelcard}

\vspace{2pt}

% Model 5: MMSearch-R1
\begin{modelcard}{accentGreen}{MMSearch-R1 (Ours)}{\verdictCorrect}
\fieldlabel{ANSWER:} \correct{B. 2 stacks}

\vspace{2pt}
\fieldlabel{REASONING:}
\textit{[Round 1]} The question asks for the maximum number of stacks in a 5-piece set effect, which depends on identifying the exact in-game mechanism. Since the image alone does not provide enough reliable evidence about the set or its stacking rule, the model first calls image search.\\[1pt]
\textit{[Round 2]} The returned visual candidates suggest the relevant element may be ``Resonance: Void Thunder,'' but the match is still not reliable enough to answer the stacking question directly. The model therefore continues with text search to verify the 5-piece effect description.\\[1pt]
\textit{[Round 3]} The retrieved text states that the 5-piece effect grants Electro DMG Bonus after certain actions, and that this effect can stack up to 2 times, each lasting 15 seconds. Therefore, the correct answer is 2 stacks.

\vspace{1pt}
\begin{retrievalGallery}
  \retrievalItemImg{R1}{IMG/CASE_SHOW/CASE1/151565282692_001.jpg}{鸣潮 合鸣·彻空冥雷}{Wuthering Waves Resonance: Void Thunder}
  \retrievalItemText{R2}%
    {Electro DMG Bonus 5-piece effect}%
    {Void Thunder (Wuthering Waves)\ldots 2-Piece: Electro DMG +10\%\ldots this effect can stack up to 2 times, with each stack lasting 15 seconds \ldots}
\end{retrievalGallery}
\end{modelcard}

\vspace{18pt}

\end{showcasebox}

\newpage

\begin{showcasebox}[Case 2]

% --- Video Information ---
\begin{subcard}{accentBlue}{\faVideo\ \ Video Information}

\fieldlabel{TITLE}\\[2pt]
\bi{怪物猎人荒野白炽龙套装展示-充能斧~原视频来自youtube，作者Pinit}%
   {Monster Hunter Wilds – Whiteflame Wyvern Armor Set Showcase | Charge Blade}

\vspace{6pt}
\fieldlabel{COVER OCR}\\[2pt]
\bi{Monster Hunter Wilds – Whiteflame Wyvern Armor Set | Charge Blade | Armor Set Showcase}%
   {《怪物猎人：荒野》白炽龙套装展示｜充能斧}

\vspace{6pt}
\fieldlabel{ASR TRANSCRIPT}\\[2pt]
\bi{N/A}{No ASR transcript available for this sample.}

\end{subcard}

\vspace{6pt}

% --- Query ---
\begin{subcard}{accentTeal}{\faQuestionCircle\ \ Query}

\begin{center}
  \includegraphics[width=0.5\linewidth]{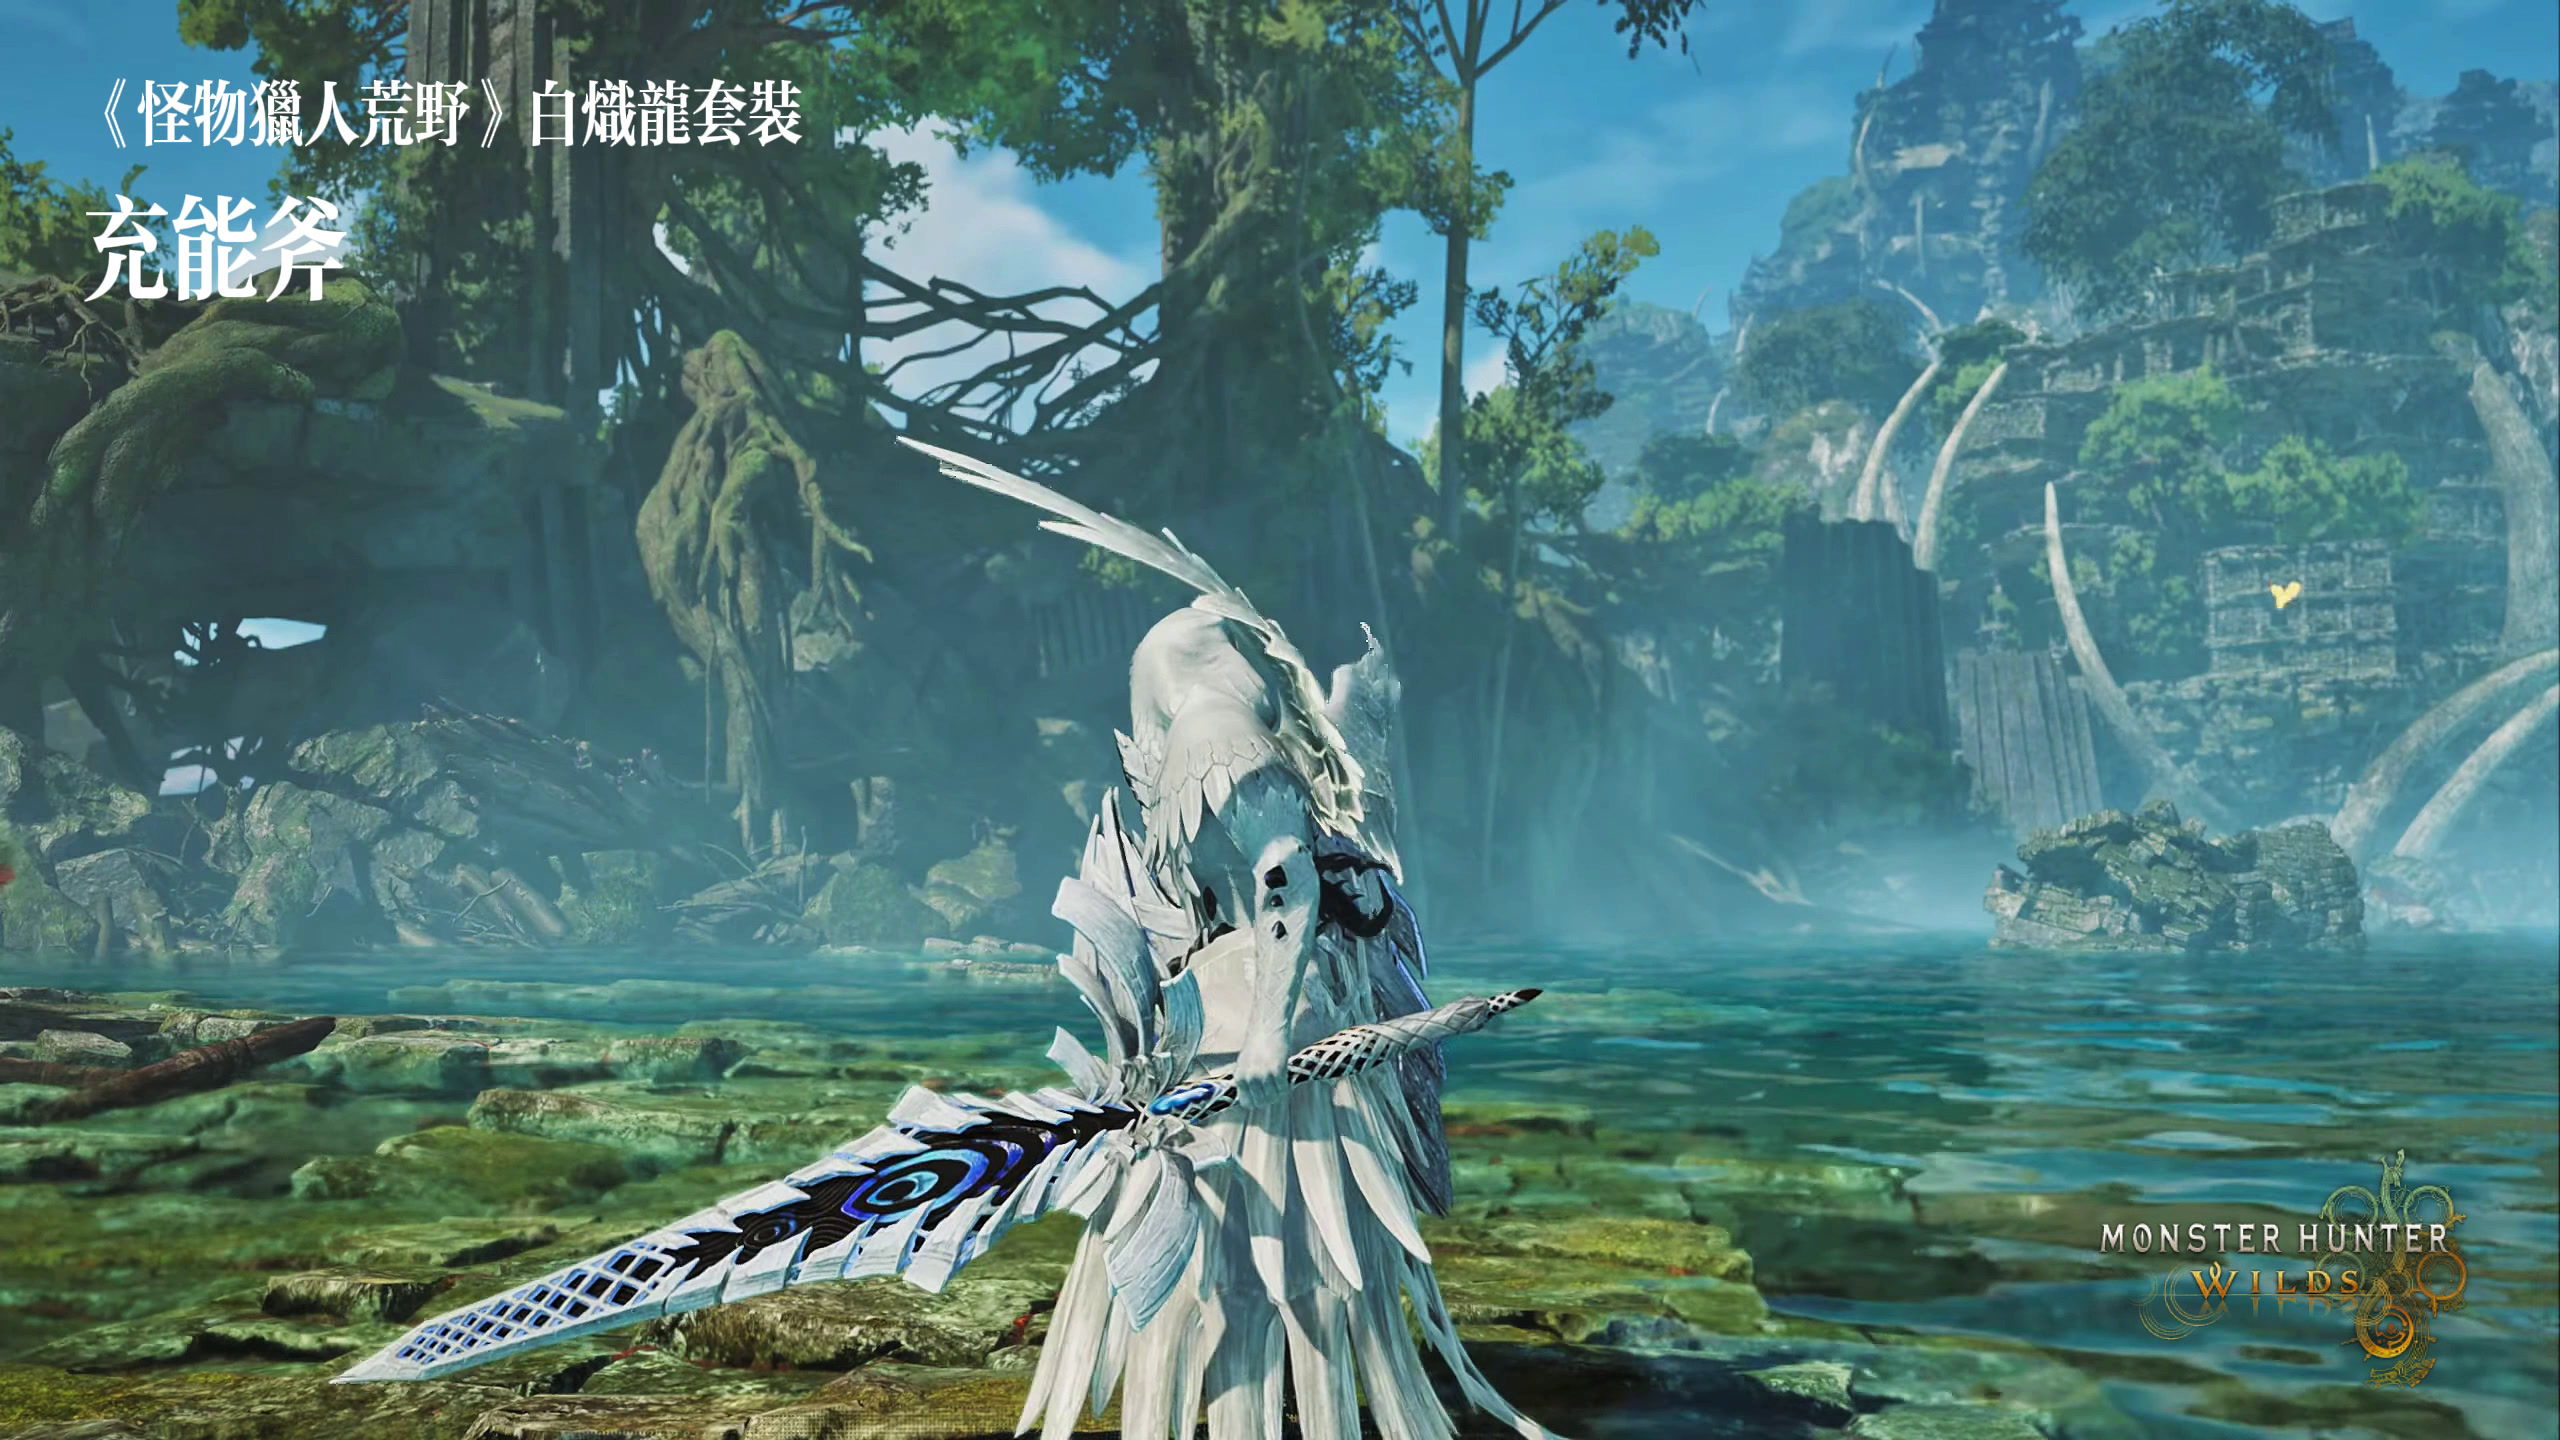}\\[2pt]
  {\footnotesize\itshape Query image}
\end{center}

\vspace{4pt}
\fieldlabel{QUESTION}\\[2pt]
\bi{充能斧在剑模式下如何为瓶子充能？}%
   {How are phials generated/charged in Sword Mode with the Charge Blade?}

\vspace{6pt}
\fieldlabel{OPTIONS}\par
\vspace{2pt}

\noindent\hspace*{0.5em}%
\begin{minipage}{\dimexpr\linewidth-1.5em\relax}
\begin{choices}
  \choice{A}{\correct{\bi{攻击敌人积累能量}{Build up energy by attacking enemies}}}
  \choice{B}{\bi{使用R+A键注入能量}{Inject energy using the R + A input}}
  \choice{C}{\bi{长按$\bigcirc$键触发GP}{Hold the Circle ($\bigcirc$) button to trigger Guard Point (GP)}}
  \choice{D}{\bi{消耗瓶子释放技能}{Consume phials to unleash attacks}}
\end{choices}
\end{minipage}

\vspace{4pt}
\fieldlabel{GROUND TRUTH}\ \ \correct{A. 攻击敌人积累能量\,/\,Build up energy by attacking enemies}

\end{subcard}

\vspace{6pt}

% --- Model Outputs ---

\newpage

\noindent\textbf{\small Model Outputs}\\[0.5pt]

% Model 1: Vanilla
\begin{modelcard}{accentGray}{Vanilla Model}{\verdictWrong}
\fieldlabel{ANSWER:} B. Inject energy using the R + A input

\vspace{1pt}
\end{modelcard}

\vspace{1pt}

% Model 2: Thinking
\begin{modelcard}{accentPurple}{Thinking Model}{\verdictWrong}
\fieldlabel{ANSWER:} B. Inject energy using the R + A input

\vspace{1pt}
\fieldlabel{REASONING:} \textit{[Thinking]} The question asks how the Charge Blade charges phials in Sword Mode\ldots However, the image provides no explicit control instructions, so the answer cannot be derived purely from visual evidence\ldots Based on typical game mechanics, charging is performed via a specific input\ldots \\[2pt]
\textit{[Final]} Therefore, option B (using the R + A input to inject energy) is selected.
\end{modelcard}

\vspace{1pt}

% Model 3: RAG
\begin{modelcard}{accentBrown}{RAG (Ours)}{\verdictCorrect}
\fieldlabel{ANSWER:} \correct{A. Build up energy by attacking enemies}

\vspace{1pt}

\begin{retrievalGallery}
  \retrievalItemImg{R1}{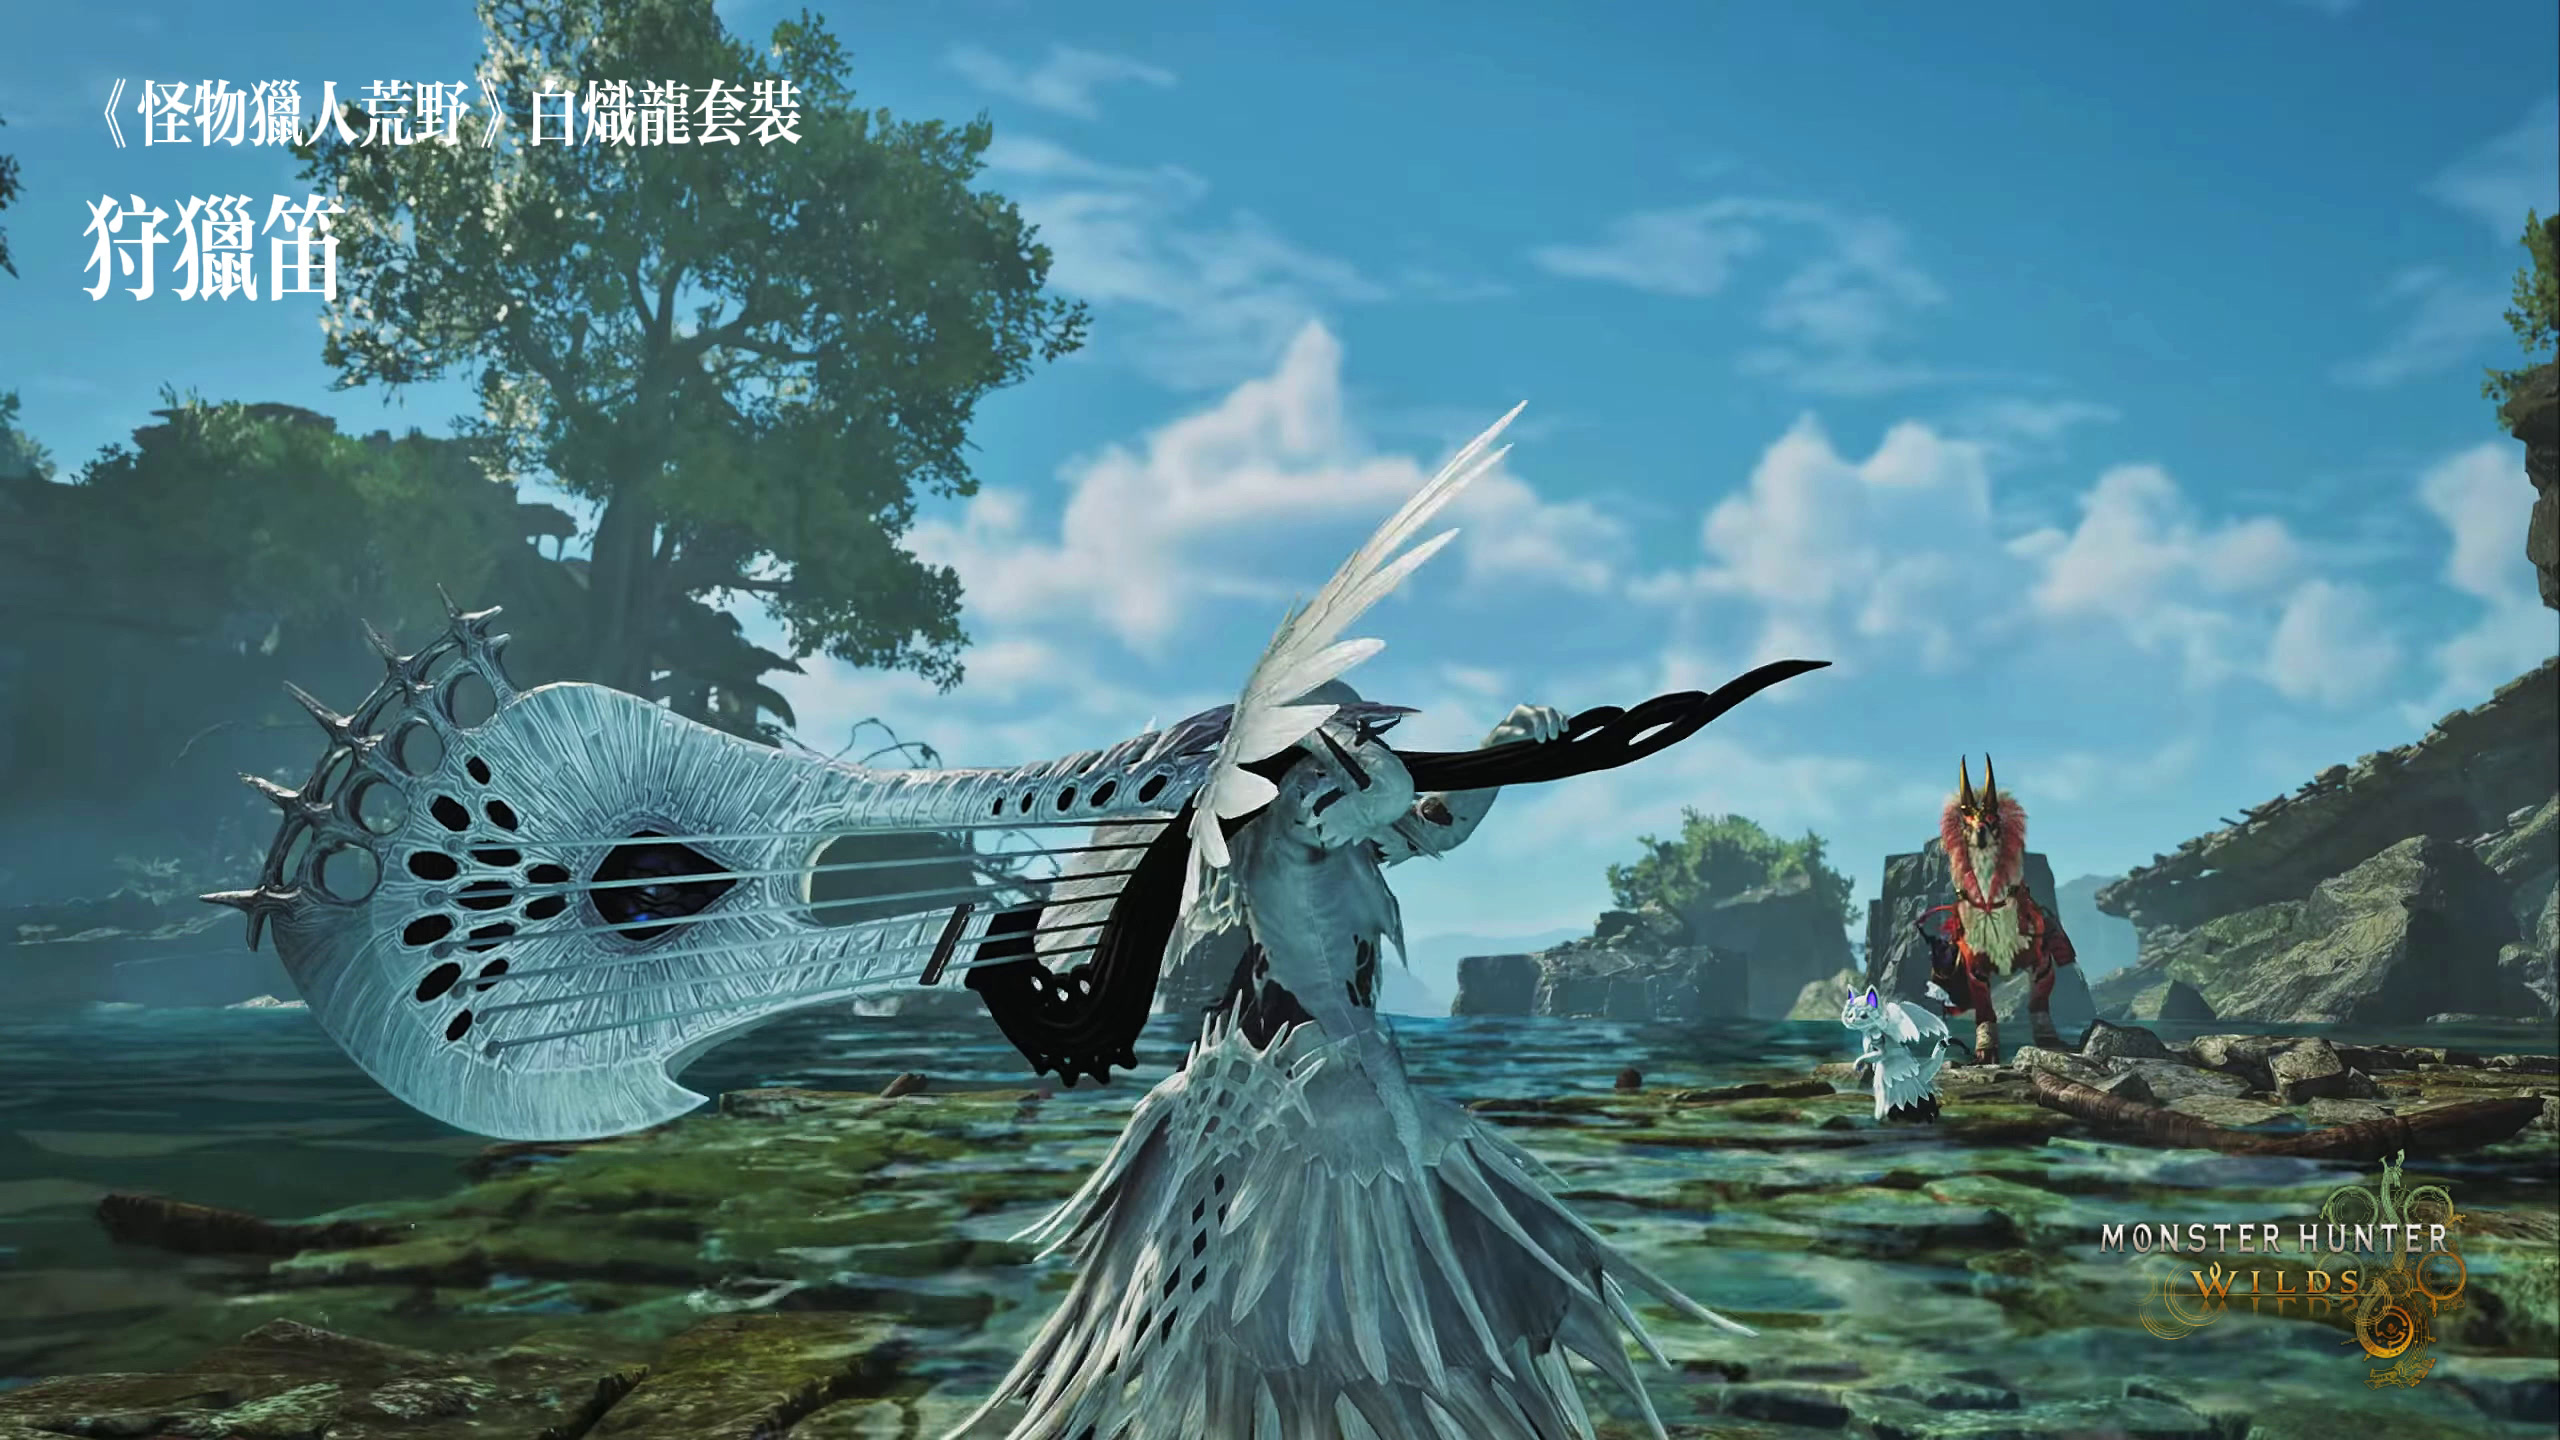}{怪物猎人\quad 狩猎笛}{Monster Hunter: Hunting Horn}
  \retrievalItemText{R2}%
    {In Monster Hunter, considering the Hunting Horn and Charge Blade, how does the Charge Blade charge phials\ldots}%
    {1) Phials are charged through sword attacks and later consumed to unleash\ldots \newline
   2) The Charge Blade is a morph weapon that switches between Sword and Axe modes, storing energy\ldots}
\end{retrievalGallery}
\end{modelcard}

\vspace{1pt}

% Model 4: LangGraph
\begin{modelcard}{accentOrange}{LangGraph (Ours)}{\verdictCorrect}
\fieldlabel{ANSWER:} \correct{A. Build up energy by attacking enemies}

\vspace{1pt}
\fieldlabel{REASONING:} 
\textit{[Plan]} Identify how phials are charged in Sword Mode…\\
\textit{[Tool: img\_ann]} Retrieve relevant Monster Hunter weapon visuals…\\
\textit{[Tool: text\_ann]} Retrieve Charge Blade mechanics… result shows phials are built up through attacks…\\
\textit{[Synthesize]} Evidence indicates energy is accumulated via attacking enemies… thus, the answer is A. Build up energy by attacking enemies.

\begin{retrievalGallery}
  \retrievalItemImg{R1}{IMG/CASE_SHOW/CASE2/162139018519_003.jpg}{怪物猎人\quad 狩猎笛}{Monster Hunter: Hunting Horn}
  \retrievalItemText{R2}%
  {How does the Charge Blade charge phials while in Sword Mode?}%
  {1) In Sword Mode, phials are charged by attacking enemies. Charging progresses in two stages: yellow and red\ldots\newline
   2) In Axe Mode, these phials can be consumed to perform Elemental Discharge attacks\ldots}
\end{retrievalGallery}
\end{modelcard}

\vspace{2pt}

% Model 5: MMSearch-R1
\begin{modelcard}{accentGreen}{MMSearch-R1 (Ours)}{\verdictCorrect}
\fieldlabel{ANSWER:} \correct{A. Build up energy by attacking enemies}

\vspace{2pt}
\fieldlabel{REASONING:}
\textit{[Round 1]} The image shows a Charge Blade in Monster Hunter Wilds, but does not provide explicit charging mechanics. The model first performs image search to identify the weapon.\\[1pt]
\textit{[Round 2]} Visual results confirm the weapon as the Charge Blade (despite some noisy matches such as Hunting Horn). However, no direct evidence about phial charging is obtained, so the model proceeds to text search.\\[1pt]
\textit{[Round 3]} Retrieved knowledge indicates that in Sword Mode, phials are charged by attacking enemies. Therefore, the correct answer is A.

\vspace{1pt}
\begin{retrievalGallery}
  \retrievalItemImg{R1}{IMG/CASE_SHOW/CASE2/162139018519_003.jpg}{怪物猎人\quad 狩猎笛}{Monster Hunter: Hunting Horn}
  \retrievalItemText{R2}%
  {Monster Hunter Wilds – Charge Blade Sword Mode phial charging method}%
  {1) The Charge Blade, also known as the Switch Axe Shield (or simply Charge Blade), is a hybrid weapon in the Monster Hunter series\ldots\newline
   2) The Charge Blade is a weapon that combines both flexibility and burst damage, and holds a prominent role in the Monster Hunter series due to its unique sword–axe switching mechanics and phial system\ldots}
\end{retrievalGallery}
\end{modelcard}

\vspace{18pt}

\end{showcasebox}
